# Supplementary material for: Synergistic interplay of morphology and metabolic activity rule response to CAR-T cells in B-cell lymphomas
Source: arXiv:2505.11894 source file (2025-05-17)
Supplement: Supplementary file 1 [file supplementary_information.pdf]

Supplementary Information for  
“Synergistic interplay of morphology and metabolic  
activity rule response to CAR-T cells in B-cell  
lymphomas”

Yifan Chen<sup>1,4†</sup>, Soukaina Sabir<sup>1,2,3†</sup>, Christina Kuttler<sup>4</sup>,  
Juan Belmonte-Beitia<sup>1,2,3</sup>, Alvaro Martínez-Rubio<sup>5</sup>,  
Lourdes Martín-Martín<sup>6</sup>, Lucía López-Corral<sup>7</sup>,  
J. Cristobal Cañadas Salazar<sup>7</sup>, Carlos Montes-Fuentes<sup>7</sup>,  
M. Pilar Tamayo-Alonso<sup>7</sup>, Angel Cedillo<sup>8</sup>, Pascual Balsalobre<sup>8</sup>,  
Pere Barba<sup>9</sup>, Antonio Pérez-Martínez<sup>10,11</sup>,  
Víctor M. Pérez-García<sup>1,2,3\*</sup>

<sup>1</sup>Mathematical Oncology Laboratory (MOLAB), Instituto de  
Matemática Aplicada a la Ciencia y la Ingeniería, University of  
Castilla-La Mancha, Spain.

<sup>2</sup>Department of Mathematics, Escuela Técnica Superior de Ingeniería  
Industrial, University of Castilla-La Mancha, Spain.

<sup>3</sup>Laboratorio de Oncología Matemática, Instituto de Investigación  
Sanitaria de Castilla-La Mancha (IDISCAM), Spain.

<sup>4</sup>Department of Mathematics, TUM School of Computation,  
Information and Technology, Technical University of Munich,  
Boltzmannstr. 3, Garching, 85747, Germany.

<sup>5</sup> Institut Curie, Paris, France.

<sup>6</sup> Universidad de Salamanca, Salamanca, Spain.

<sup>7</sup> Hospital Universitario de Salamanca, Instituto de Investigación  
Biomédica de Salamanca (IBSAL), Salamanca, Spain.

<sup>8</sup> Grupo Español de Trasplante Hematopoyético y Terapia Celular,  
Madrid, Spain.

<sup>9</sup> Hospital Universitari Vall d’Hebron, Barcelona, Spain.

<sup>10</sup> University Hospital La Paz, Madrid, Spain.

<sup>11</sup> Great Ormond Street Hospital for Children, London, United Kingdom.

\*Corresponding author(s). E-mail(s): [victor.perezgarcia@uclm.es](mailto:victor.perezgarcia@uclm.es);

<sup>†</sup>These authors contributed equally to this work.

## Contents

|          |                                                     |           |
|----------|-----------------------------------------------------|-----------|
| <b>1</b> | <b>Supplementary Figures</b>                        | <b>3</b>  |
| <b>2</b> | <b>Patient data</b>                                 | <b>3</b>  |
| 2.1      | Study design . . . . .                              | 3         |
| <b>3</b> | <b>Statistical analysis</b>                         | <b>5</b>  |
| 3.1      | Model selection . . . . .                           | 5         |
| 3.2      | Effect of treatment type . . . . .                  | 9         |
| <b>4</b> | <b>Supplementary note: Mathematical Analysis</b>    | <b>12</b> |
| 4.1      | Nondimensionalization of the model . . . . .        | 12        |
| 4.2      | Equilibria and nullclines . . . . .                 | 12        |
| 4.3      | Local stability . . . . .                           | 18        |
| <b>5</b> | <b>Supplementary tables: Data used in the study</b> | <b>22</b> |

# 1 Supplementary Figures

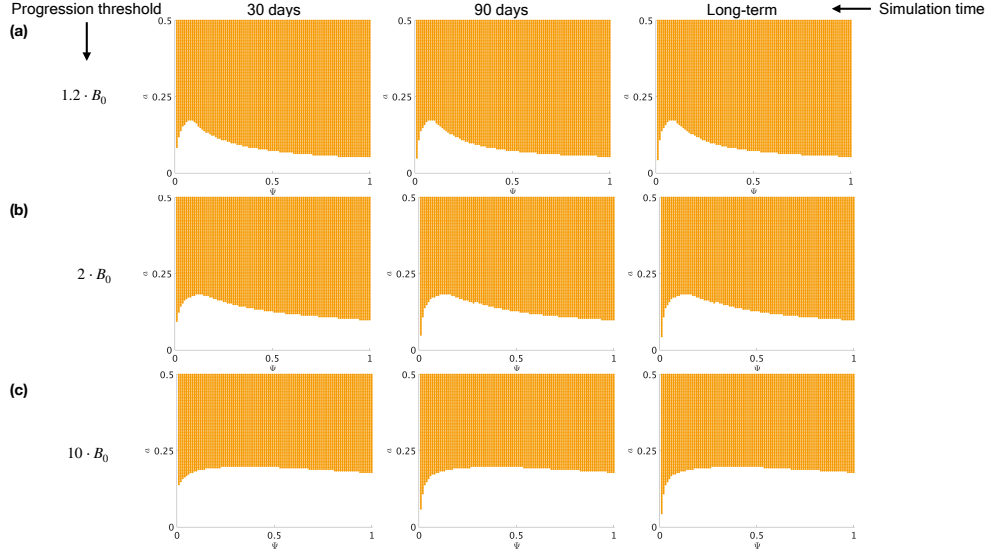

**Fig. S1: Impact of proliferation rate ( $a$ ) and lesion sphericity ( $\Psi$ ) on the dynamics of tumor cell population ( $B$ ) depending on the simulation time and the threshold used to define progressive disease.** Initial tumor cell population ( $B_0$ ) and CAR T-cell does ( $C_0$ ) are given in Table 2. For each set of parameter combination  $a$  and  $\Psi$ , we ran model simulations within different time spans (columns) using different upper bound on the tumor cell population used to define a disease progression (rows). Color dots are parameter combinations for which a disease progression (row) occurs within the simulation time span (column).

## 2 Patient data

### 2.1 Study design

The patient selection process is outlined in figure S2. Initially, 78 patients were considered; however, 9 were excluded because pre-infusion PET scans were not performed or unavailable, likely due to logistical issues or patient condition at the time of imaging. Another three patients were excluded due to technical problems with PET scan segmentation, which affected the accuracy of tumor data, rendering these scans unusable. Additionally, three patients diagnosed with mantle cell lymphoma (MCL), a different subtype treated with Tecartus (KTE-C19), were also excluded. In total, 63 patients met the final inclusion criteria for our analysis.

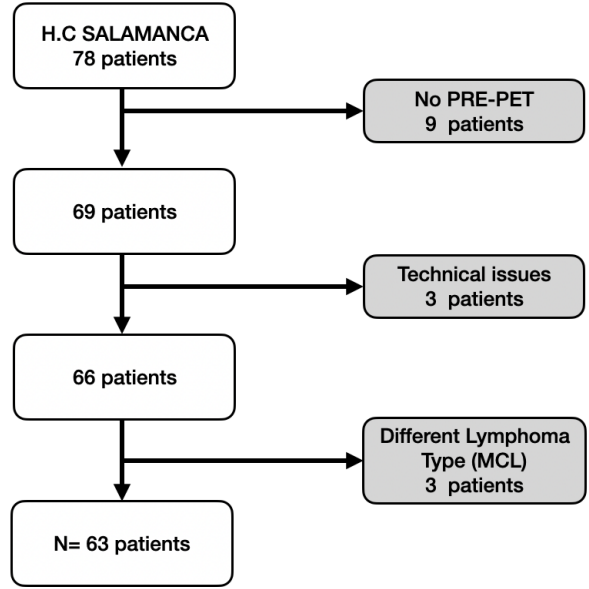

**Fig. S2:** Flow diagram depicting the patient selection process for the study conducted at the Clinical Hospital of Salamanca. Patients were excluded based on missing pre-infusion PET scans, technical issues, or a different lymphoma subtype ((Mantle Cell Lymphoma, MCL). N represents the final eligible patient count for analysis.

Thus, our cohort comprised 63 individuals, as detailed in table S8, all diagnosed with aggressive non-Hodgkin B-cell lymphoma. Among these patients, 73% were diagnosed with diffuse large B-cell lymphoma (DLBCL), while the remaining patients had high-grade B-cell lymphoma, primary mediastinal large B-cell lymphoma, transformed follicular lymphoma, or composite lymphoma. The CAR-T products approved by the U.S. Food and Drug Administration (FDA) for the treatment of large B-cell lymphoma include Axicabtagene ciloleucel (axi-cel), developed by Kite Pharma, and Tisagenlecleucel (tisa-cel), produced by Novartis. In our cohort, 68% of the patients received axi-cel, while 31% were treated with tisa-cel.

Notably, 15.9% of patients had undergone autologous stem cell transplant (ASCT) prior to CAR-T therapy, a strategy often employed to maintain disease control in individuals with chemosensitive relapses before transitioning to CAR-T as a salvage therapy.

As CAR-T therapy is indicated for relapsed or refractory cases, all patients in this cohort had received prior treatments. The majority (84.13%) had undergone two lines of therapy, while 15.87% had received more than two lines.

Bridge therapy, implemented to control disease progression during the CAR-T cell manufacturing period, was administered to 74.6% of patients. Among those who received bridge therapy, 61% were treated with chemotherapy alone or in combination with radiotherapy and immunotherapy (such as monoclonal antibodies). In contrast, some patients received corticosteroids or radiotherapy alongside immunotherapy. The

use of bridge therapy is not universal; it depends on factors such as the patient’s disease stability and overall health. Patients may not require bridge therapy if their disease remains stable during the manufacturing process or if they are deemed too frail to tolerate additional treatments. In our cohort, 25.4% did not receive bridge therapy due to these clinical considerations or other contraindications.

Regarding treatment response, early treatment response to CAR-T therapy was evaluated within the first three months post-infusion. Of the 63 patients treated, 57.14% ( $n = 36$ ) demonstrated a response, defined as either complete response (CR) or partial response (PR). CR refers to the total disappearance of all signs of disease following treatment, with no evidence of residual tumors on imaging or clinical examination. PR, on the other hand, indicates a clear reduction in the extent of disease, though some detectable tumor remains. Notably, 71% of these responders achieved CR within the first month following CAR-T infusion. Among those who attained an initial CR, 56% sustained their remission for up to 18 months post-infusion, highlighting the potential for durable long-term efficacy in a subset of patients. Additionally, four patients who initially exhibited a PR at one month post-infusion converted to CR by day 90, underscoring the dynamic nature of early CAR-T responses. However, disease progression was observed in 38.09% ( $n = 24$ ) of patients during this early evaluation period. Of note, six patients who initially responded experienced disease progression by day 90 during the second evaluation, while two additional patients experienced late progression, one at six months and the other at 18 months post-infusion. Additionally, one patient did not undergo a response evaluation within 90 days because the PET scan was not performed.

### 3 Statistical analysis

#### 3.1 Model selection

Figure S3 shows the Kaplan-Meier (KM) plot of the progression-free survival after the CAR T-cell infusion. The median time progression-free survival time is 149 days, while the median follow-up time is 720 days after the CAR T-cell infusion.

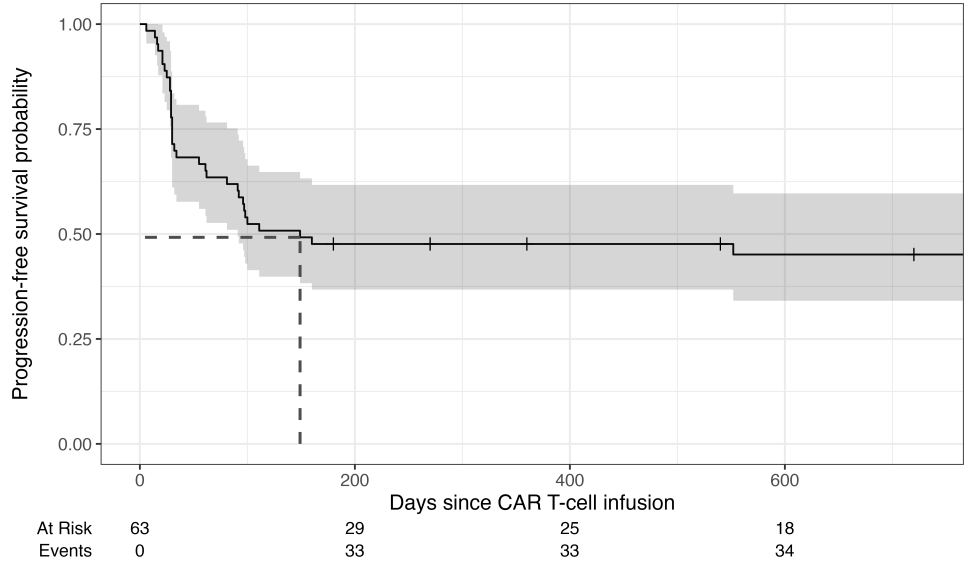

**Fig. S3:** Kaplan-Meier curve showing progression-free survival probability over time. The solid black line represents the estimated survival function, while the shaded region indicates the 95% confidence interval. The number of patients at risk and the number of events at different time points are displayed below the plot.

We begin with assessing a full model containing the features. Table S1 shows the results for the multivariate Cox Proportional Hazard (PH) model. The Likelihood-ratio test of the model is given by 14.7 with a p-value of 0.1. We observe that the covariates total TLG, total MTV, volume of lesion with largest sphericity, and volume of lesion with smallest sphericity have a (HR) of 1.000. We exclude these features.

**Table S1:** Result of the multivariate Cox regression analysis for PFS including all covariates. The Likelihood-ratio statistic is given by 14.7 (on 9 degrees of freedom) with a p-value of 0.1. HR = Hazard Ratio, CI = Confidence Interval

| Covariate                                      | HR     | p-value | 95% CI           |
|------------------------------------------------|--------|---------|------------------|
| tTLG                                           | 1.000  | 0.609   | 1.000 - 1.000    |
| Total MTV                                      | 1.000  | 0.649   | 1.000 - 1.000    |
| Maximum SUV                                    | 1.012  | 0.720   | 0.949 - 1.079    |
| Largest sphericity                             | 22.478 | 0.233   | 0.135 - 3745.650 |
| Volume of lesion with largest sphericity       | 1.000  | 0.734   | 1.000 - 1.000    |
| Maximum SUV of lesion with largest sphericity  | 1.011  | 0.734   | 0.951 - 1.075    |
| Smallest sphericity                            | 0.786  | 0.863   | 0.051 - 12.171   |
| Volume of lesion with smallest sphericity      | 1.000  | 0.340   | 1.000 - 1.000    |
| Maximum SUV of lesion with smallest sphericity | 1.052  | 0.127   | 0.986 - 1.122    |

For the remaining features, Figure S4 shows the Spearman correlation coefficients. We observe that the maximum SUV (SUVmax) and the maximum SUV of the lesion with the smallest sphericity (SUVmaxMinSpher) have a correlation coefficient of 0.72. Keeping in mind that in the full model, the HR of SUVmax is 1.012 with a p-value of 0.720 and thus, we also exclude this covariate.

The resulting Cox PH model including the largest sphericity (maxSpher), maximum SUV of lesion with largest sphericity (SUVmaxMaxSpher), smallest sphericity (minSpher), and maximum SUV of lesion with smallest sphericity (SUVmaxMinSpher) yields a Likelihood-ratio of 13.470 on 4 degrees of freedom, the p-value is given by 0.009. We observe that the global significance has improved compared to the full model. Further, the p-value of the covariate SUVmaxMinSpher is given by 0.029.

The result of the univariate Cox regression analysis using only the covariate SUVmaxMinSpher is given in Table S3 with a p-value  $< 0.001$ . We compare the later two models by assuming for the Null hypothesis that the coefficients for the covariates largest sphericity (maxSpher), maximum SUV of lesion with largest sphericity (SUVmaxMaxSpher), and smallest sphericity (minSpher) are zero. The partial log-likelihoods for the model in Table S2 and in Table S3 are given by  $-122.5603$  and  $-123.8347$ , respectively. The likelihood statistic is thus,  $2(-122.5603 + 123.8347) = 2.5488$ . Comparing this to a chi-square distribution with  $4 - 1 = 3$  degrees of freedom yields a p-value of 0.467 and we thus choose the univariate model with only the covariate SUVmaxMinSpher.

**Table S2:** Result of the multivariate Cox regression analysis for PFS including only maxSpher, SUVmaxMaxSpher, minSpher, SUVmaxMinSpher. The Likelihood-ratio statistics is given by 13.47 (on 4 degrees of freedom) with a p-value of 0.009. The log-likelihood is given by  $-122.5603$ . HR = Hazard Ratio, CI = Confidence Interval

|                                                | HR     | p-value | 95% CI          |
|------------------------------------------------|--------|---------|-----------------|
| Covariate                                      |        |         |                 |
| Largest sphericity                             | 14.167 | 0.149   | 0.387 - 518.607 |
| Maximum SUV of lesion with largest sphericity  | 1.015  | 0.602   | 0.959 - 1.075   |
| Smallest sphericity                            | 0.801  | 0.825   | 0.111 - 5.760   |
| Maximum SUV of lesion with smallest sphericity | 1.054  | 0.029   | 1.005 - 1.105   |

**Table S3:** Result of the univariate Cox regression analysis for PFS. The Likelihood-ratio statistic is given by 10.92 with a p-value of 0.001. The log-likelihood is given by  $-123.8347$ . HR = Hazard Ratio, CI = Confidence Interval

|                                                | HR    | p-value   | 95% CI        |
|------------------------------------------------|-------|-----------|---------------|
| Covariate                                      |       |           |               |
| Maximum SUV of lesion with smallest sphericity | 1.060 | $< 0.001$ | 1.026 - 1.096 |

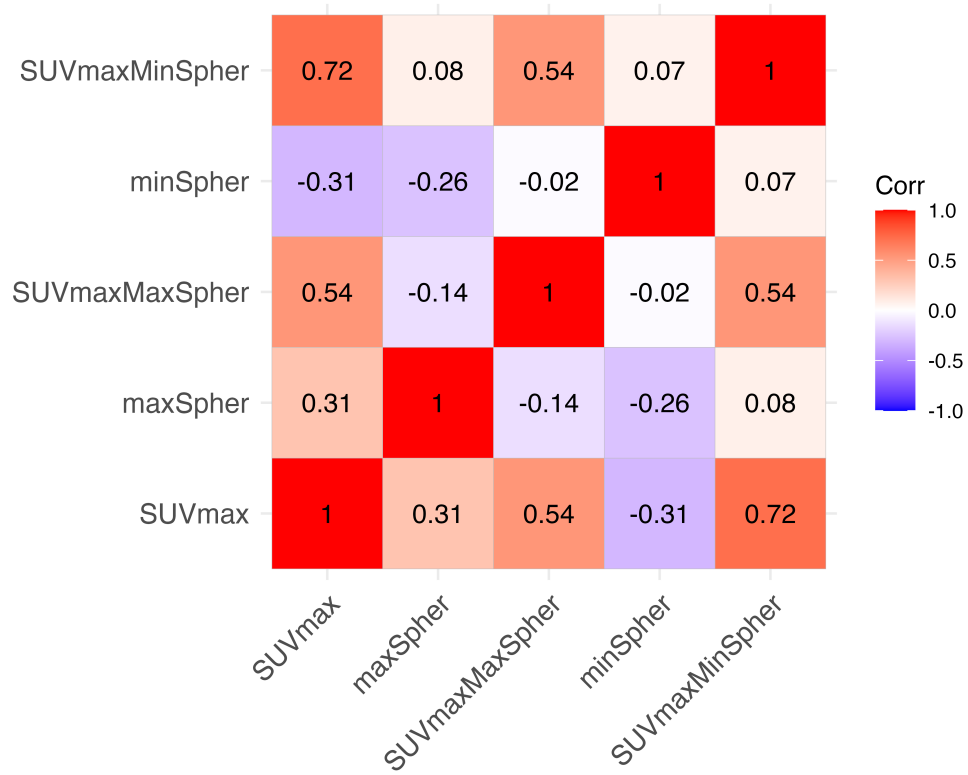

**Fig. S4:** Correlation matrix of quantitative PET imaging parameters. The heatmap displays the Spearman correlation coefficients between SUVmax, maxSpher, SUVmaxMaxSpher, minSpher, and SUVmaxMinSpher. Positive correlations are shown in red, while negative correlations are shown in blue, with intensity reflecting the strength of the correlation.

We further computed the scaled Schoenfeld residuals for the covariate SUVmaxMinSpher to test the PH assumption using the “correlation with time” test. Figure S5 shows the estimate of the time-dependent coefficient. We observe that the smooth curve is fairly level across the time horizon here and with a p-value of 0.183, we can assume no significant change in the effect of SUVmaxMinSpher over time.

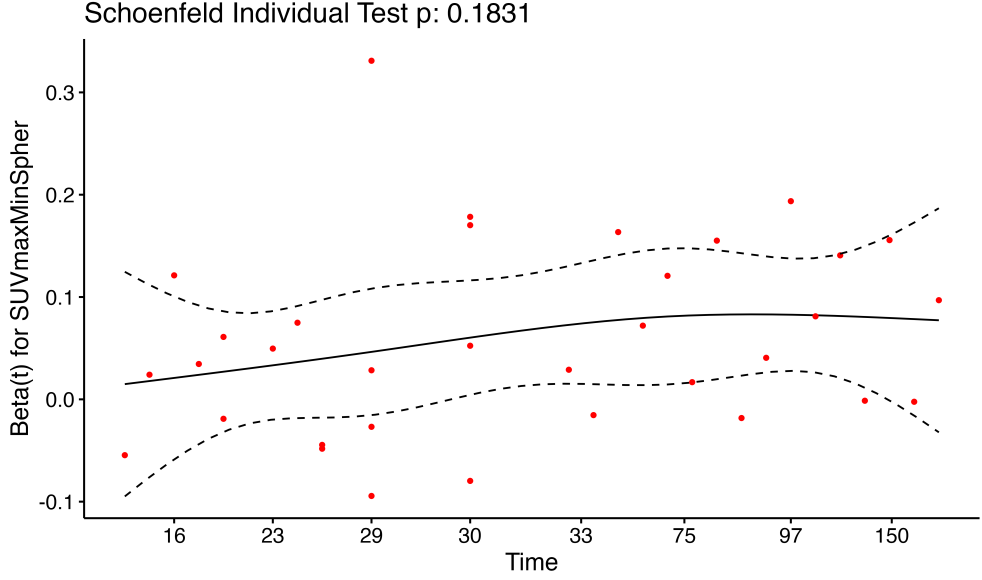

**Fig. S5:** Estimate of the time-dependent coefficient  $\beta(t)$  for the covariate SUVmaxMinSpher. The solid line represents the overall trend, with red points indicating individual patient data. The Schoenfeld individual test yields a p-value of 0.1813, suggesting no significant difference.

### 3.2 Effect of treatment type

To assess whether treatment type adds prognostic value beyond the effect of SUVmaxMinSpher, we further compared a model including both covariates, i.e. treatment type and SUVmaxMinSpher, to the univariate model including only SUVmaxMinSpher. The results of the multivariate model are given in Table S4. The log-likelihood for the model including the treatment type is  $-122.3963$ . It follows that the likelihood statistic is  $2(-122.3963 + 123.8347) = 2.8768$ . Comparing this to a chi-square distribution with  $2 - 1 = 1$  degree of freedom yields a p-value of 0.090. On a level of 0.05, we conclude that adding treatment type does not significantly improve model fit after adjusting for SUVmaxMinSpher.

**Table S4:** Result of the multivariate Cox regression analysis for PFS including SUVmaxMinSpher and treatment type. The Likelihood-ratio statistic is given by 13.80 (on 2 degrees of freedom) with a p-value 0.001. The log-likelihood is given by  $-122.3963$ . HR = Hazard Ratio, CI = Confidence Interval

|                                                | HR    | p-value | 95% CI        |
|------------------------------------------------|-------|---------|---------------|
| Covariate                                      |       |         |               |
| Maximum SUV of lesion with smallest sphericity | 1.056 | 0.001   | 1.022 - 1.091 |
| Treatment type                                 | 1.837 | 0.084   | 0.922 - 3.660 |

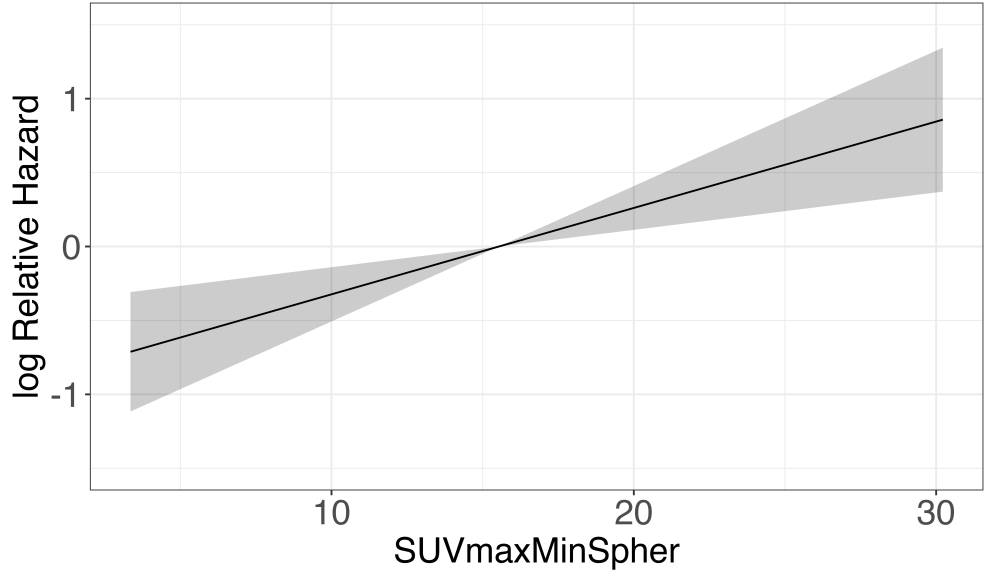

**Fig. S6:** Fitted effect of SUVmaxMinSpher on the log hazard of progression. The plot illustrates the estimated relationship between SUVmaxMinSpher and the log relative hazard of disease progression, with the solid line representing the estimated effect and the shaded region indicating the 95 % confidence interval.

Figure S6 shows the effect of SUVmaxMinSpher on the log relative hazard. We see that a higher maximum SUV of the most irregular lesion is associated with a higher log relative hazard. Figure S7 shows the survival curves for above and below the 0.25, 0.5, and 0.75 quantile of the covariate SUVmaxMinSpher. We observe that patients with a higher diagnosis SUVmaxMinSpher tend to have a lower PFS probability with increasing time.

The effect of comparing SUVmaxMinSpher at the 0.25 quantile (SUVmaxMinSpher = 8.61) to SUVmaxMinSpher at the 0.75 quantile (SUVmaxMinSpher = 21.26) yielded a hazard ratio of 2.09 (95% CI: 1.377 - 3.183). This suggests that patients with higher SUVmaxMinSpher values (by approximately 12.65 units) have more than twice the risk of progression compared to those with lower SUVmaxMinSpher values.

Additionally, the per-unit effect size of the covariate SUVmaxMinSpher corresponds to a hazard ratio of approximately 1.06, suggesting a 6% increase in the hazard of progression for each unit increase in the SUVmaxMinSpher value.

Among patients who had no progression/relapse until the end of the study or the time of their lost of follow-up, five of them died and were previously censored. In a “worst-case scenario”, we assume that these deaths correspond to progression events occurring at the time of death. We then fit a univariate Cox PH model using SUVmaxMinSpher as the only covariate. Table S5 shows the result of the corresponding model. The Likelihood ratio test yields a p-value of 0.002, suggesting that the

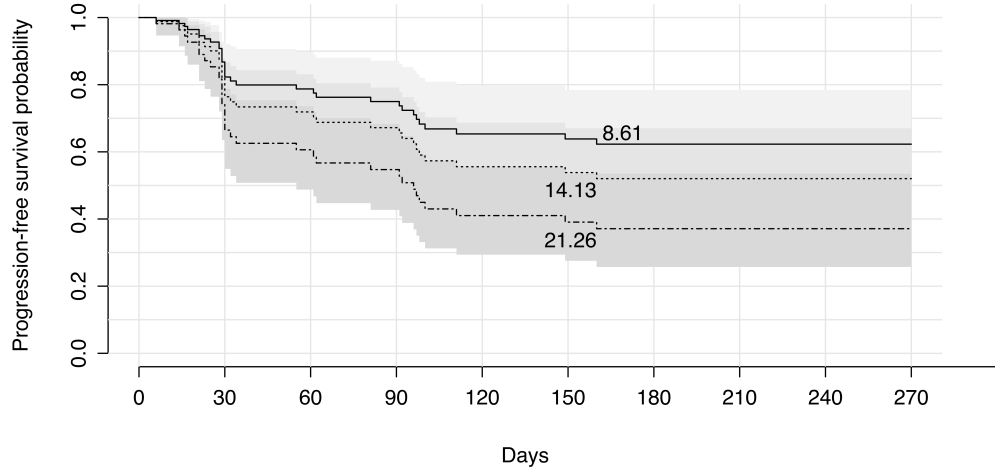

**Fig. S7:** Kaplan-Meier progression-free survival curves stratified by SUVmaxMinSpher quartiles. The curves represent the progression-free survival probabilities for patients grouped according to the 0.25 (dashed-dotted line), 0.5 (dashed line), and 0.75 (solid line) quartiles of SUVmaxMinSpher, with shaded regions indicating 95% confidence intervals.

association between SUVmaxMinSpher and the PFS remains statistically significant on a level of 0.05.

**Table S5:** Result of the univariate Cox regression analysis for PFS in the “worst case scenario”. The Likelihood-ratio statistic is given by 9.18 with a p-value 0.002. The log-likelihood is given by  $-140.0413$ . HR = Hazard Ratio, CI = Confidence Interval

|                                                | HR    | p-value | 95% CI        |
|------------------------------------------------|-------|---------|---------------|
| Covariate                                      |       |         |               |
| Maximum SUV of lesion with smallest sphericity | 1.053 | 0.002   | 1.020 - 1.087 |

## 4 Supplementary note: Mathematical Analysis

### 4.1 Nondimensionalization of the model

Following [1], we nondimensionalize the system by considering  $x := bB$ ,  $y := bC$ , and  $\tau := at$ . We associate  $dx/d\tau$  and  $dy/d\tau$  with  $\dot{x}$  and  $\dot{y}$ , respectively and denote  $\bar{d} := \frac{1}{ab^{2/3}}\Psi^{-1}d$ ,  $\bar{q} := \frac{1}{ab^{2/3}}\Psi^{-1}q$ ,  $\bar{g} := \frac{b}{(\Psi^{-1})^{3/2}}g$ ,  $\bar{j} := \frac{1}{a}j$ , and  $\bar{m} := \frac{1}{a}m$  leading to the nondimensionalized model

$$\dot{x} = x(1-x) - \bar{d}x^{2/3}y, \quad (1a)$$

$$\dot{y} = -\bar{q}x^{2/3}y + \frac{\bar{j}x^{2/3}}{\bar{g}^{2/3} + x^{2/3}}y - \bar{m}y. \quad (1b)$$

For simplicity, we drop the bars of the parameters  $\bar{d}, \bar{q}, \bar{j}, \bar{g}$ , and  $\bar{m}$  for the rest of the work and keep in mind that these are dimensionless parameters. We observe that the set  $D := [0, 1] \times [0, \infty) \subset \mathbb{R}^2$  is positively invariant for the system (1) for all  $n > 0$ , as

$$\begin{aligned} x = 0, y \geq 0 : \quad \dot{x} &= 0, \\ x = 1, y \geq 0 : \quad \dot{x} &= -dy \leq 0, \\ y = 0, x \in [0, 1] : \quad \dot{y} &= 0. \end{aligned}$$

### 4.2 Equilibria and nullclines

The equilibria are found by determining the intersections of the nullclines  $\dot{x} = 0$  and  $\dot{y} = 0$  in  $D$ . The nullclines are given by

$$\dot{x} = 0 : \quad x = 0 \quad \text{or} \quad y = \frac{1-x}{dx^{-1/3}} =: f_1(x), \quad (2a)$$

$$\dot{y} = 0 : \quad y = 0 \quad \text{or} \quad f_2(x) := -qx^{2/3} + \frac{jx^{2/3}}{g^{2/3} + x^{2/3}} - m = 0. \quad (2b)$$

Note that the equilibria  $E_0 = (\bar{x}_0, \bar{y}_0) = (0, 0)$  and  $E_3 = (\bar{x}_3, \bar{y}_3) = (1, 0)$  always exist. The steady state  $E_3$  can be considered as the tumor-escape scenario while the steady state  $E_0$  can be described as the tumor-free equilibrium. Note that the first equation in (1) is not differentiable in  $x = 0$ . Therefore, it is not possible to study the stability of this equilibrium  $E_0$  by determining the eigenvalues of the linearized system around  $E_0$ . However, we note that for  $y = 0$  and  $x > 0$ ,  $\dot{x} = x(1-x)$  is always positive. It thus follows that  $E_0$  is unstable regardless of the parameter values chosen.

If  $f_1$  is well-defined on the entire interval  $(0, 1)$ , which is the case here, then the non-trivial equilibria are given by  $(\bar{x}, \bar{y})$ , where  $\bar{x} \in (0, 1)$  is a solution of  $f_2(x) = 0$  on the interval  $(0, 1)$  and  $\bar{y} = f_1(\bar{x})$ . The following lemma allows us to determine the number of solutions of  $f_2(x) = 0$  in  $(0, 1)$ .

**Lemma 1.** Let  $q, j, g$ , and  $m$  be positive, and consider

$$f_2(x) = -qx^{2/3} + \frac{jx^{2/3}}{g^{2/3} + x^{2/3}} - m. \quad (3)$$

If  $mg^{2/3} < q$  and

- $j < qg^{2/3} + m + 2\sqrt{qg^{2/3}m}$ , then  $f_2$  has no roots in  $(0, 1)$ ;
- $j = qg^{2/3} + m + 2\sqrt{qg^{2/3}m}$ , then  $f_2$  has one root in  $(0, 1)$ ;
- $qg^{2/3} + m + 2\sqrt{qg^{2/3}m} < j < qg^{2/3} + m + q + mg^{2/3} = (1 + g^{2/3})(q + m)$ , then  $f_2$  has 2 roots in  $(0, 1)$ ;
- $j \geq (1 + g^{2/3})(q + m)$ , then  $f_2$  has one root in  $(0, 1)$ .

If  $mg^{2/3} \geq q$  and

- $j \leq (1 + g^{2/3})(q + m)$ , then  $f_2$  has no roots in  $(0, 1)$ ;
- $j > (1 + g^{2/3})(q + m)$ , then  $f_2$  has one root in  $(0, 1)$ .

Further, for  $x \in (\bar{x}_1, \bar{x}_2)$ ,  $f_2(x) > 0$  and for  $x \notin (\bar{x}_1, \bar{x}_2)$ , we have that  $f_2(x) < 0$ .

*Proof.* Let  $z := x^{2/3}$ . For  $f_2(x) = 0$ , we have the chain of equivalences

$$\begin{aligned} & -qx^{2/3} + \frac{jx^{2/3}}{g^{2/3} + x^{2/3}} - m = 0 \\ \Leftrightarrow & -qx^{4/3} + (-qg^{2/3} - m + j)x^{2/3} - mg^{2/3} = 0 \\ \Leftrightarrow & z^2 - \frac{-qg^{2/3} - m + j}{q}z + \frac{mg^{2/3}}{q} = 0 \\ \Leftrightarrow & z_{1,2} = \frac{-qg^{2/3} - m + j \pm \sqrt{(-qg^{2/3} - m + j)^2 - 4qg^{2/3}m}}{2q}. \end{aligned}$$

Note that  $z \in (0, 1)$  iff  $x \in (0, 1)$  and with  $\bar{x}_{1,2} = z_{1,2}^{1/n}$ , there are at most two roots in  $(0, 1)$ . We now analyze the conditions for which  $z_{1,2} \in (0, 1)$  is satisfied. The solutions  $z_{1,2}$  are real iff

$$\begin{aligned} 0 & \leq (-qg^{2/3} - m + j)^2 - 4qg^{2/3}m \\ & = (j^2 - 2(qg^{2/3} + m)j + (qg^{2/3})^2 + m^2 + 2qg^{2/3}m) - 4qg^{2/3}m \\ & = j^2 - 2(qg^{2/3} + m)j + (qg^{2/3})^2 + m^2 - 2qg^{2/3}m \\ & = j^2 - 2(qg^{2/3} + m)j + (qg^{2/3} - m)^2 \end{aligned} \quad (4)$$

is satisfied. For fixed parameters  $q, g^{2/3}, m$  and variable  $j$ , this is a parabola facing upward. Thus, (4) is fulfilled for all  $0 < j \leq j_1$  and  $j_2 \leq j$ , where

$$\begin{aligned} j_{1,2} & = qg^{2/3} + m \pm \sqrt{(qg^{2/3} + m)^2 - (qg^{2/3} - m)^2} \\ & = qg^{2/3} + m \pm 2\sqrt{qg^{2/3}m}. \end{aligned}$$

The second equality follows from

$$\begin{aligned}(qg^{2/3} + m)^2 - (qg^{2/3} - m)^2 &= (qg^{2/3})^2 + 2qg^{2/3}m + m^2 - (qg^{2/3})^2 + 2qg^{2/3}m - m^2 \\ &= 4qg^{2/3}m.\end{aligned}$$

We first have a look at the case where  $mg^{2/3} < q$ , and consider the scenarios

- (a)  $0 < j < qg^{2/3} + m - 2\sqrt{qg^{2/3}m}$ ,
- (b)  $j = qg^{2/3} + m - 2\sqrt{qg^{2/3}m}$ ,
- (c)  $j = qg^{2/3} + m + 2\sqrt{qg^{2/3}m}$ ,
- (d)  $qg^{2/3} + m + 2\sqrt{qg^{2/3}m} < j < qg^{2/3} + m + q + mg^{2/3} = (1 + g^{2/3})(q + m)$ ,
- (e)  $j = (1 + g^{2/3})(q + m)$ , and
- (f)  $j > (1 + g^{2/3})(q + m)$ .

Recall that Scenario (a)-(f) guarantee that  $z_1$  and  $z_2$  are real. We will later also consider the same scenarios for  $mg^{2/3} \geq q$ . Note that for  $mg^{2/3} \neq q$ , we have  $q + mg^{2/3} - 2\sqrt{qg^{2/3}m} = (\sqrt{q} - \sqrt{mg^{2/3}})^2 > 0$ , which implies that  $qg^{2/3} + m + 2\sqrt{qg^{2/3}m} < qg^{2/3} + m + q + mg^{2/3}$ . Therefore, Scenario (d) is possible. On the other hand,  $mg^{2/3} = q$  implies that  $2\sqrt{qg^{2/3}m} = 2q = q + mg^{2/3}$  and thus, Scenario (c) and (e) fall together and Scenario (d) will never appear. We observe the following for  $mg^{2/3} < q$ :

**Scenario (a)**

We have

$$\frac{-qg^{2/3} - m + j}{2q} < -\frac{2\sqrt{qg^{2/3}m}}{2q} = -\sqrt{\frac{mg^{2/3}}{q}} < 0$$

and  $\sqrt{(-qg^{2/3} - m + j)^2 - 4qg^{2/3}m} < qg^{2/3} + m - j$ . It follows that  $z_1, z_2 < 0$  and thus,  $f_2$  has no roots in  $(0, 1)$ .

**Scenario (b)**

We have

$$z_1 = z_2 = \frac{-qg^{2/3} - m + j}{2q} = -\frac{2\sqrt{qg^{2/3}m}}{2q} = -\sqrt{\frac{mg^{2/3}}{q}} < 0$$

and thus,  $f_2$  has no roots in  $(0, 1)$ .

**Scenario (c)**

With

$$0 < z_1 = z_2 = \frac{-qg^{2/3} - m + j}{2q} = \frac{2\sqrt{qg^{2/3}m}}{2q} = \sqrt{\frac{mg^{2/3}}{q}} < 1,$$

$f_2$  has one root in  $(0, 1)$ .

**Scenario (d)**

With  $\sqrt{(-qg^{2/3} - m + j)^2 - 4qg^{2/3}m} < -qg^{2/3} - m + j$  and  $-qg^{2/3} - m + j > 2\sqrt{qg^{2/3}m} > 0$ , we have  $z_1, z_2 > 0$ . Further, with  $-qg^{2/3} - m + j < q + mg^{2/3}$ , it follows that

$$\begin{aligned}
& q(-qg^{2/3} - m + j) < q(q + mg^{2/3}) = q^2 + qg^{2/3}m \\
\Leftrightarrow & 4q(-qg^{2/3} - m + j) < 4q^2 + 4qg^{2/3}m \\
\Leftrightarrow & -4qg^{2/3}m < 4q^2 - 4q(-qg^{2/3} - m + j) \\
\Leftrightarrow & (-qg^{2/3} - m + j)^2 - 4qg^{2/3}m < 4q^2 - 4q(-qg^{2/3} - m + j) + (-qg^{2/3} - m + j)^2 \\
\Leftrightarrow & (-qg^{2/3} - m + j)^2 - 4qg^{2/3}m < (2q - (-qg^{2/3} - m + j))^2.
\end{aligned}$$

Since  $2q - (-qg^{2/3} - m + j) > 2q - q - mg^{2/3} = q - mg^{2/3} > 0$  holds true, we have

$$\begin{aligned}
& \sqrt{(-qg^{2/3} - m + j)^2 - 4qg^{2/3}m} < 2q - (-qg^{2/3} - m + j) \\
\Leftrightarrow & -qg^{2/3} - m + j + \sqrt{(-qg^{2/3} - m + j)^2 - 4qg^{2/3}m} < 2q \\
\Leftrightarrow & z_2 = \frac{-qg^{2/3} - m + j + \sqrt{(-qg^{2/3} - m + j)^2 - 4qg^{2/3}m}}{2q} < 1.
\end{aligned}$$

and particularly, since  $z_1 < z_2$  holds,  $z_1 < 1$  holds true as well. Therefore,  $z_{1,2}$  are both in  $(0, 1)$  and  $f_2$  has two roots in  $(0, 1)$ .

**Scenario (e)**

With  $\sqrt{(-qg^{2/3} - m + j)^2 - 4qg^{2/3}m} < -qg^{2/3} - m + j$  and  $-qg^{2/3} - m + j = q + mg^{2/3} > 0$ , we have  $z_1, z_2 > 0$ . Further, we observe that  $(-qg^{2/3} - m + j)^2 - 4qg^{2/3}m = (q + mg^{2/3})^2 - 4qg^{2/3}m = (q - mg^{2/3})^2$  and since  $mg^{2/3} < q$  holds, we have

$$\begin{aligned}
z_1 &= \frac{-qg^{2/3} - m + j - q + mg^{2/3}}{2q} = \frac{q + mg^{2/3} - q + mg^{2/3}}{2q} = \frac{mg^{2/3}}{q} < 1, \\
z_2 &= \frac{-qg^{2/3} - m + j + q - mg^{2/3}}{2q} = \frac{q + mg^{2/3} + q - mg^{2/3}}{2q} = 1.
\end{aligned}$$

Thus,  $f_2$  has one root in  $(0, 1)$ .

**Scenario (f)**

With  $\sqrt{(-qg^{2/3} - m + j)^2 - 4qg^{2/3}m} < -qg^{2/3} - m + j$  and  $-qg^{2/3} - m + j > q + mg^{2/3} > 0$ , we have  $z_1, z_2 > 0$ . Further, with  $-(-qg^{2/3} - m + j) < -q - mg^{2/3}$ , we have

$$\begin{aligned}
& -4q(-qg^{2/3} - m + j) < -4q^2 - 4qg^{2/3}m \\
\Leftrightarrow & (-qg^{2/3} - m + j)^2 - 4q(-qg^{2/3} - m + j) + 4q^2 < (-qg^{2/3} - m + j)^2 - 4qg^{2/3}m \\
\Leftrightarrow & ((-qg^{2/3} - m + j) - 2q)^2 < (-qg^{2/3} - m + j)^2 - 4qg^{2/3}m.
\end{aligned}$$

With  $\sqrt{(-qg^{2/3} - m + j)^2 - 4qg^{2/3}m} > |(-qg^{2/3} - m + j) - 2q| \geq (-qg^{2/3} - m + j) - 2q$ , it follows that

$$\begin{aligned}
& \sqrt{(-qg^{2/3} - m + j)^2 - 4qg^{2/3}m} > (-qg^{2/3} - m + j) - 2q \\
\Leftrightarrow & -\sqrt{(-qg^{2/3} - m + j)^2 - 4qg^{2/3}m} < -(-qg^{2/3} - m + j) + 2q \\
\Leftrightarrow & (-qg^{2/3} - m + j) - \sqrt{(-qg^{2/3} - m + j)^2 - 4qg^{2/3}m} < 2q \\
\Leftrightarrow & z_1 = \frac{(-qg^{2/3} - m + j) - \sqrt{(-qg^{2/3} - m + j)^2 - 4qg^{2/3}m}}{2q} < 1.
\end{aligned}$$

On the other hand, with  $\sqrt{(-qg^{2/3} - m + j)^2 - 4qg^{2/3}m} > |(-qg^{2/3} - m + j) - 2q| \geq -(-qg^{2/3} - m + j) + 2q$ , we have

$$\begin{aligned}
& \sqrt{(-qg^{2/3} - m + j)^2 - 4qg^{2/3}m} > -(-qg^{2/3} - m + j) + 2q \\
\Leftrightarrow & (-qg^{2/3} - m + j) + \sqrt{(-qg^{2/3} - m + j)^2 - 4qg^{2/3}m} > 2q \\
\Leftrightarrow & z_2 = \frac{(-qg^{2/3} - m + j) + \sqrt{(-qg^{2/3} - m + j)^2 - 4qg^{2/3}m}}{2q} > 1.
\end{aligned}$$

Thus,  $f_2$  has one root in  $(0, 1)$ .

We note that the arguments for Scenario (a), (b), and (f) do not depend on the relation between  $q$  and  $mg^{2/3}$  and can be performed in an analogous way for  $mg^{2/3} \geq q$ .

For  $mg^{2/3} = q$ , we have the following:

**Scenario (c) and (e)**

We have

$$z_1 = z_2 = \frac{-qg^{2/3} - m + j}{2q} = \frac{2q}{2q} = 1$$

and thus,  $f_2$  has no roots in  $(0, 1)$ .

Lastly, for  $mg^{2/3} > q$ , we have the following:

**Scenario (c)**

We have

$$z_1 = z_2 = \frac{-qg^{2/3} - m + j}{2q} = \frac{2\sqrt{qg^{2/3}m}}{2q} = \sqrt{\frac{mg^{2/3}}{q}} > 1.$$

Thus,  $f_2$  has no roots in  $(0, 1)$ .

**Scenario (d)**

Similar as before, we have

$$4q(-qg^{2/3} - m + j) < 4q^2 + 4qg^{2/3}m$$

$$\begin{aligned}
&\Leftrightarrow (-qg^{2/3} - m + j)^2 - 4qg^{2/3}m < (-qg^{2/3} - m + j)^2 - 4q(-qg^{2/3} - m + j) + 4q^2 \\
&\Leftrightarrow (-qg^{2/3} - m + j)^2 - 4qg^{2/3}m < (2q - (-qg^{2/3} - m + j))^2.
\end{aligned}$$

and since  $2\sqrt{qg^{2/3}m} < -qg^{2/3} - m + j < q + mg^{2/3}$  and  $mg^{2/3} > q$  hold true, we observe that

$$2q - (-qg^{2/3} - m + j) < 2q - 2\sqrt{qg^{2/3}m} < 2q - 2q = 0,$$

which leads to

$$\begin{aligned}
&\sqrt{(-qg^{2/3} - m + j)^2 - 4qg^{2/3}m} < (-qg^{2/3} - m + j) - 2q \\
&\Leftrightarrow -\sqrt{(-qg^{2/3} - m + j)^2 - 4qg^{2/3}m} > -(-qg^{2/3} - m + j) + 2q \\
&\Leftrightarrow (-qg^{2/3} - m + j) - \sqrt{(-qg^{2/3} - m + j)^2 - 4qg^{2/3}m} > 2q \\
&\Leftrightarrow z_1 = \frac{(-qg^{2/3} - m + j) - \sqrt{(-qg^{2/3} - m + j)^2 - 4qg^{2/3}m}}{2q} > 1.
\end{aligned}$$

Since  $z_2 > z_1 > 1$ ,  $f_2$  has no roots in  $(0, 1)$ .

### Scenario (e)

We observe that  $(-qg^{2/3} - m + j)^2 - 4qg^{2/3}m = (q + mg^{2/3})^2 - 4qg^{2/3}m = (mg^{2/3} - q)^2$  and since  $mg^{2/3} > q$  holds true, we have

$$\begin{aligned}
z_1 &= \frac{-qg^{2/3} - m + j - mg^{2/3} + q}{2q} = \frac{q + mg^{2/3} - mg^{2/3} + q}{2q} = \frac{q}{q} = 1, \\
z_2 &= \frac{-qg^{2/3} - m + j + mg^{2/3} - q}{2q} = \frac{q + mg^{2/3} + mg^{2/3} - q}{2q} = \frac{mg^{2/3}}{q} > 1.
\end{aligned}$$

Hence,  $f_2$  has no roots in  $(0, 1)$ .

From the previous analysis, we can have the following cases for the position of the roots  $\bar{x}_{1,2}$ , where  $\bar{x}_1 \leq \bar{x}_2$ :

- $\bar{x}_{1,2} \leq 0$ ,
- $\bar{x}_1 \in (0, 1)$  and  $\bar{x}_2 \geq 1$ ,
- $\bar{x}_{1,2} \in (0, 1)$ , and
- $\bar{x}_{1,2} \geq 1$ .

Furthermore, we note that  $f_2$  is continuous in  $[0, 1]$ , where  $f_2(0) = -m < 0$ . A change of sign occurs only at  $\bar{x}_{1,2}$  and since  $\bar{x}_1 \leq \bar{x}_2$ , we have that  $f_2(x) > 0$  for  $x \in (\bar{x}_1, \bar{x}_2)$ . In particular, for  $\bar{x}_{1,2} \leq 0$  and  $\bar{x}_{1,2} \geq 1$ ,  $f_2(x) < 0$  for all  $x \in (0, 1)$ .  $\square$

We can now formulate the following theorem on the number of equilibria of system (1) in  $\text{int}(D)$ .

**Theorem 1.** Let  $n, d, q, j, g$ , and  $m$  be positive and consider the system (1). Let  $f_1$  be the non-zero component of the  $x$  nullcline. If  $f_1 : (0, 1) \rightarrow [0, \infty)$  is well-defined, then the following holds. If  $mg^{2/3} < q$  and

- $j < qg^{2/3} + m + 2\sqrt{qg^{2/3}m}$ , then system (1) has no equilibria in  $\text{int}(D)$ ;
- $j = qg^{2/3} + m + 2\sqrt{qg^{2/3}m}$ , then system (1) has one additional equilibrium in  $\text{int}(D)$ ;
- $qg^{2/3} + m + 2\sqrt{qg^{2/3}m} < j < qg^{2/3} + m + q + mg^{2/3} = (1 + g^{2/3})(q + m)$ , then system (1) has two additional equilibria in  $\text{int}(D)$ ;
- $j \geq (1 + g^{2/3})(q + m)$ , then system (1) has one additional equilibrium in  $\text{int}(D)$ .

If  $mg^{2/3} \geq q$  and

- $j \leq (1 + g^{2/3})(q + m)$ , then system (1) has no additional equilibria in  $\text{int}(D)$ ;
- $j > (1 + g^{2/3})(q + m)$ , then system (1) has one additional equilibrium in  $\text{int}(D)$ .

*Proof.* From Lemma 1, we know the number of roots of  $f_2$  in  $(0, 1)$  and since  $f_1$  in (2) is defined on the interval  $(0, 1)$ , we have

$$\bar{y}_{1,2} = \frac{1 - \bar{x}_{1,2}}{d\bar{x}_{1,2}^{-\frac{1}{3}}} > 0$$

if  $\bar{x}_{1,2} \in (0, 1)$ , where  $\bar{x}_{1,2}$  are the roots of  $f_2$ . □

### 4.3 Local stability

We denote the non-trivial equilibria as  $E_{1,2} = (\bar{x}_{1,2}, \bar{y}_{1,2})$ , where  $\bar{x}_1 < \bar{x}_2$  and  $\bar{y}_{1,2} = \frac{1 - \bar{x}_{1,2}}{d\bar{x}_{1,2}^{-\frac{1}{3}}}$ . For the linearized system of (1), the general Jacobian matrix for  $x > 0$  reads

$$J(x, y) = \begin{pmatrix} 1 - 2x - \frac{2}{3}dx^{-1/3}y & -dx^{2/3} \\ -\frac{2}{3}qx^{-1/3}y + \frac{2}{3}g^{2/3}\frac{jx^{-1/3}}{(g^{2/3}+x^{2/3})^2}y - qx^{2/3} + \frac{jx^{2/3}}{g^{2/3}+x^{2/3}} - m \end{pmatrix}.$$

For  $(x, y) = (1, 0) = E_3$ , we have

$$J(1, 0) = \begin{pmatrix} -1 & -d \\ 0 & -q + \frac{j}{g^{2/3}+1} - m \end{pmatrix}.$$

The eigenvalues are given by  $-1$  and  $-q + \frac{j}{g^{2/3}+1} - m$ . Since we have excluded  $j = (1 + g^{2/3})(q + m)$  earlier, the eigenvalues have a non-zero real part. In particular,  $E_3$  is locally asymptotically stable, if

$$-q + \frac{j}{g^{2/3}+1} - m < 0$$

is satisfied, which is equivalent to

$$j < (q + m)(g^{2/3} + 1) = qg^{2/3} + m + q + mg^{2/3}.$$

As we have seen previously, this implies the case where there are either no or two additional equilibria in  $\text{int}(D)$ . If  $(q+m)(g^{2/3}+1) < j$  holds true, then the system (1) has only one additional equilibrium in  $\text{int}(D)$  and  $E_3$  becomes unstable. For a non-trivial equilibrium  $(\bar{x}, \bar{y}) \in \{E_1, E_2\}$ , we have that

$$\begin{aligned} J(\bar{x}, \bar{y}) &= \begin{pmatrix} 1 - 2\bar{x} - \frac{2}{3}d\bar{x}^{-1/3}\bar{y} & -d\bar{x}^{2/3} \\ -\frac{2}{3}q\bar{x}^{-1/3}\bar{y} + \frac{2}{3}\frac{jg^{2/3}\bar{x}^{-1/3}}{(g^{2/3}+\bar{x}^{2/3})^2}\bar{y} & 0 \end{pmatrix} \\ &= \begin{pmatrix} 1 - 2\bar{x} - \frac{2}{3}(1-\bar{x}) & -dz \\ \frac{2}{3}\frac{1-\bar{x}}{d}\left(-q + \frac{jg^{2/3}}{(g^{2/3}+z)^2}\right) & 0 \end{pmatrix}, \end{aligned}$$

where  $z = \bar{x}^{2/3}$ . The corresponding characteristic equation reads

$$\lambda^2 - (1 - 2\bar{x} - \frac{2}{3}(1-\bar{x})) \cdot \lambda + \frac{2}{3}z(1-\bar{x}) \left(-q + \frac{jg^{2/3}}{(g^{2/3}+z)^2}\right) = 0,$$

which yields the eigenvalues

$$\begin{aligned} \lambda_1(\bar{x}) &= \frac{1 - 2\bar{x} - \frac{2}{3}(1-\bar{x})}{2} \\ &\quad - \frac{\sqrt{(1 - 2\bar{x} - \frac{2}{3}(1-\bar{x}))^2 - 4\frac{2}{3}z(1-\bar{x}) \left(-q + \frac{jg^{2/3}}{(g^{2/3}+z)^2}\right)}}{2}, \\ \lambda_2(\bar{x}) &= \frac{1 - 2\bar{x} - \frac{2}{3}(1-\bar{x})}{2} \\ &\quad + \frac{\sqrt{(1 - 2\bar{x} - \frac{2}{3}(1-\bar{x}))^2 - 4\frac{2}{3}z(1-\bar{x}) \left(-q + \frac{jg^{2/3}}{(g^{2/3}+z)^2}\right)}}{2}. \end{aligned}$$

We now study the stability of the equilibria  $E_1$  and  $E_2$  in the following theorem.

**Theorem 2.** *Consider the system (1) and assume the parameters to be chosen in such a way that  $1 - 2z_1^{3/2} - \frac{2}{3}(1 - z_1^{3/2}) < 0$ . If  $E_1 \in \text{int}(D)$ , then it is locally asymptotically stable. If  $E_2 \in \text{int}(D)$ , then it is unstable.*

*Proof.* We begin with the equilibrium  $E_1 \in \text{int}(D)$ . For  $\lambda_1(\bar{x}_1)$ , we observe that the real part is, by assumption, always negative. Further,  $\text{Re}(\lambda_2(\bar{x}_1)) < 0$  is fulfilled iff

$$\begin{aligned} &\left(1 - 2\bar{x}_1 - \frac{2}{3}(1 - \bar{x}_1)\right)^2 - 4\frac{2}{3}z_1(1 - \bar{x}_1) \left(-q + \frac{jg^{2/3}}{(g^{2/3} + z_1)^2}\right) \\ &< \left(1 - 2\bar{x}_1 - \frac{2}{3}(1 - \bar{x}_1)\right)^2 \end{aligned}$$

is satisfied. Since  $4\frac{2}{3}z_1(1 - \bar{x}_1) > 0$ , this is equivalent to

$$-q + \frac{jg^{2/3}}{(g^{2/3} + z_1)^2} > 0. \quad (5)$$

Since  $E_1 \in \text{int}(D)$ , Theorem 1 yields  $j > qg^{2/3} + m + 2\sqrt{qg^{2/3}m}$  and hence, we have  $C := -qg^{2/3} - m + j > 0$ . With the expression for  $z_1$  derived in the proof of Lemma 1, we have

$$\begin{aligned} (g^{2/3} + z_1)^2 &= \left( \frac{2qg^{2/3} + (-qg^{2/3} - m + j) - \sqrt{(-qg^{2/3} - m + j)^2 - 4qg^{2/3}m}}{2q} \right)^2 \\ &= \left( \frac{2qg^{2/3} + C - \sqrt{C^2 - 4qg^{2/3}m}}{2q} \right)^2 \end{aligned}$$

and it follows that

$$-q + \frac{jg^{2/3}}{(g^{2/3} + z_1)^2} = \frac{-q \left( 2qg^{2/3} + C - \sqrt{C^2 - 4qg^{2/3}m} \right)^2 + 4q^2 jg^{2/3}}{\left( 2qg^{2/3} + C - \sqrt{C^2 - 4qg^{2/3}m} \right)^2},$$

which has the same sign as

$$\begin{aligned} & - \left( 2qg^{2/3} + C - \sqrt{C^2 - 4qg^{2/3}m} \right)^2 + 4qjg^{2/3} \\ &= - \left( 4q^2 \left( g^{2/3} \right)^2 + C^2 + C^2 - 4qg^{2/3}m + 4qg^{2/3}C - 4qg^{2/3}\sqrt{C^2 - 4qg^{2/3}m} \right. \\ & \quad \left. - 2C\sqrt{C^2 - 4qg^{2/3}m} \right) + 4qjg^{2/3}, \end{aligned}$$

since  $q > 0$ . We recall that  $C = -qg^{2/3} - m + j$ , which leads to

$$\begin{aligned} & -4q^2 \left( g^{2/3} \right)^2 - 2C^2 + 4qg^{2/3}m - 4qg^{2/3}C + 4qg^{2/3}\sqrt{C^2 - 4qg^{2/3}m} + 2C\sqrt{C^2 - 4qg^{2/3}m} \\ & + 4qjg^{2/3} \underbrace{-4qg^{2/3}m + 4qg^{2/3}m}_{=0} \\ &= 4qg^{2/3}(-qg^{2/3} - m + j) - 4qg^{2/3}C - 2C^2 + 8qg^{2/3}m + 4qg^{2/3}\sqrt{C^2 - 4qg^{2/3}m} + 2C\sqrt{C^2 - 4qg^{2/3}m} \\ &= -2C^2 + 8qg^{2/3}m + 4qg^{2/3}\sqrt{C^2 - 4qg^{2/3}m} + 2C\sqrt{C^2 - 4qg^{2/3}m} \\ &= 2 \left( -C^2 + 4qg^{2/3}m + 2qg^{2/3}\sqrt{C^2 - 4qg^{2/3}m} + C\sqrt{C^2 - 4qg^{2/3}m} \right). \end{aligned}$$

We can see that

$$\begin{aligned}
& - \underbrace{(C^2 - 4qg^{2/3}m)}_{>0 \text{ since } j > qg^{2/3} + m + 2\sqrt{qg^{2/3}m}} + 2qg^{2/3}\sqrt{C^2 - 4qg^{2/3}m} + C\sqrt{C^2 - 4qg^{2/3}m} \\
& = - \left( \sqrt{C^2 - 4qg^{2/3}m} \right)^2 + 2qg^{2/3}\sqrt{C^2 - 4qg^{2/3}m} + C\sqrt{C^2 - 4qg^{2/3}m} \\
& = \sqrt{C^2 - 4qg^{2/3}m} \left( 2qg^{2/3} + \underbrace{C - \sqrt{C^2 - 4qg^{2/3}m}}_{>C-C=0} \right) > 0
\end{aligned}$$

and thus, (5) is satisfied, which yields the local asymptotic stability of  $E_1$ .

Next, we consider the case where  $E_2$  is also in  $\text{int}(D)$ . By Theorem 1, this is only the case if  $mg^{2/3} < q$  and  $qg^{2/3} + m + 2\sqrt{qg^{2/3}m} < j < qg^{2/3} + m + q + mg^{2/3}$ . In particular, this implies  $C > 0$ .

In the following, we will prove the instability of  $E_2$  by showing that

$$-q + \frac{jg^{2/3}}{(g^{2/3} + z_2)^2} < 0,$$

which implies  $\text{Re}(\lambda_2(\bar{x}_2)) > 0$ . Following the same calculations as before, we see that

$$-q + \frac{jg^{2/3}}{(g^{2/3} + z_2)^2}$$

has the same sign as

$$\begin{aligned}
& -2C^2 + 8qg^{2/3}m - 4qg^{2/3}\sqrt{C^2 - 4qg^{2/3}m} - 2C\sqrt{C^2 - 4qg^{2/3}m} \\
& = \sqrt{C^2 - 4qg^{2/3}m}(-2C - 4qg^{2/3}) + 8qg^{2/3}m - 2C^2,
\end{aligned}$$

which is smaller than zero, as  $8qg^{2/3}m - 2C^2 < 0$  since  $C^2 > 4qg^{2/3}m$ . It follows that  $\text{Re}(\lambda_2(\bar{x}_2)) > 0$  and that  $E_2$  is unstable.  $\square$

In particular, if  $E_2 \in \text{int}(D)$ , the equilibrium  $E_2$  is an unstable saddle. With  $\bar{x}_1 < \bar{x}_2$ , the stable equilibrium  $E_1 \in \text{int}(D)$  corresponds to the dormant state. If we recall the three phases of cancer immunoediting, we find that the equilibrium  $E_0$  would correspond to the elimination phase, where the tumor cell population is successfully destructed. The equilibrium phase can be represented by the non-trivial equilibrium  $E_1$ , in which the tumor cell population is kept in a dormant state. Lastly, the equilibrium  $E_3$  describes the escape phase, which is characterized by the progressive growth of tumor cell populations. Following the stability analysis, we observe that the equilibrium  $E_0$  is always unstable, which would mean that the CAR T-cell therapy is never able to destroy tumor cells completely.

## 5 Supplementary tables: Data used in the study

The tables in this study provide a comprehensive overview of tumor characteristics, CAR T-cell response parameters, and quantitative PET imaging metrics for individual patients. They include processed data on tumor burden and CAR T-cell dynamics over time ([S8](#), [S7](#), and [S6](#)), as well as parameter estimation results describing key proliferation and dynamic properties ([S9](#) and [S10](#)). Additionally, Table [S11](#), [S12](#), and [S13](#) present quantitative PET imaging metrics, capturing metabolic activity, volumetric properties, spherical tumor characteristics, and progression-free survival. Together, these data provide a robust foundation for evaluating tumor progression and treatment response.

**Table S6:** Processed data summary: Tumor characteristics and CAR T-cell response. The table includes initial tumor burden ( $B_0$ ) and estimated CAR T-cell quantification at different time points (days 0, 7, 14, 21, and 28) in number of cells. Tumor sphericity properties are also reported: propMinSpher (proportion of the tumor volume with the minimum sphericity), cellMinSpher (number of tumor cells corresponding to the lowest observed sphericity), minSpher (minimum recorded sphericity value), and SUVmaxMinSpher (maximum standardized uptake value for the lesion with the lowest sphericity). Additionally, the overall progression status (PS) is provided, where 1 indicates progression and 0 indicates no progression. Missing values in the original dataset were handled using the method described in Section (4.4). Patients 1 to 27 are listed here.

| ID  | $B_0$ (cells)        | $C_0$ (cells)     | day7 (cells)      | day14 (cells)     | day21 (cells)     | day28 (cells)     | propMinSpher | cellsMinSpher        | minSpher | PS | SUVmaxMinSpher |
|-----|----------------------|-------------------|-------------------|-------------------|-------------------|-------------------|--------------|----------------------|----------|----|----------------|
| 001 | $1.11 \cdot 10^{10}$ | $4.11 \cdot 10^8$ | $1.74 \cdot 10^7$ | $3.98 \cdot 10^7$ | 0                 | 0                 | 1.000        | $1.11 \cdot 10^{10}$ | 0.671    | 1  | 31.14          |
| 002 | $1.69 \cdot 10^{10}$ | $2.75 \cdot 10^8$ | $5.29 \cdot 10^6$ | $8.71 \cdot 10^7$ | $1.97 \cdot 10^8$ | $6.52 \cdot 10^8$ | 0.362        | $6.10 \cdot 10^9$    | 0.658    | 1  | 30.32          |
| 004 | $1.46 \cdot 10^{11}$ | $2.89 \cdot 10^8$ | 0                 | 0                 | 0                 | 0                 | 0.142        | $2.07 \cdot 10^{10}$ | 0.495    | 1  | 14.13          |
| 005 | $1.11 \cdot 10^{11}$ | $3.05 \cdot 10^8$ | $1.77 \cdot 10^8$ | $2.63 \cdot 10^8$ | $5.16 \cdot 10^7$ | $3.45 \cdot 10^7$ | 0.660        | $7.30 \cdot 10^{10}$ | 0.537    | 0  | 29.34          |
| 006 | $1.54 \cdot 10^9$    | $3.01 \cdot 10^8$ | $3.03 \cdot 10^8$ | $9.77 \cdot 10^7$ | $1.10 \cdot 10^7$ | $6.89 \cdot 10^6$ | 0.553        | $8.50 \cdot 10^8$    | 0.602    | 0  | 8.40           |
| 007 | $1.75 \cdot 10^{10}$ | $2.73 \cdot 10^8$ | $1.40 \cdot 10^7$ | $1.55 \cdot 10^9$ | $2.46 \cdot 10^8$ | $7.52 \cdot 10^7$ | 0.045        | $7.93 \cdot 10^8$    | 0.568    | 0  | 5.35           |
| 008 | $7.78 \cdot 10^{10}$ | $3.95 \cdot 10^8$ | $7.25 \cdot 10^8$ | $2.43 \cdot 10^8$ | $3.93 \cdot 10^7$ | $4.46 \cdot 10^6$ | 0.019        | $1.46 \cdot 10^9$    | 0.394    | 0  | 7.59           |
| 009 | $7.00 \cdot 10^9$    | $4.16 \cdot 10^8$ | $3.42 \cdot 10^8$ | $3.94 \cdot 10^7$ | $6.52 \cdot 10^6$ | $7.96 \cdot 10^6$ | 0.288        | $2.01 \cdot 10^9$    | 0.816    | 0  | 4.08           |
| 010 | $2.95 \cdot 10^{10}$ | $4.57 \cdot 10^8$ | 0                 | $1.28 \cdot 10^7$ | 0                 | 0                 | 0.553        | $1.63 \cdot 10^{10}$ | 0.510    | 1  | 23.88          |
| 011 | $5.44 \cdot 10^{10}$ | $2.15 \cdot 10^8$ | $1.08 \cdot 10^9$ | $2.30 \cdot 10^8$ | 0                 | 0                 | 0.016        | $8.93 \cdot 10^8$    | 0.328    | 0  | 8.91           |
| 012 | $4.01 \cdot 10^{11}$ | $3.58 \cdot 10^8$ | $8.42 \cdot 10^8$ | $2.44 \cdot 10^9$ | $1.10 \cdot 10^9$ | $3.94 \cdot 10^8$ | 0.346        | $1.39 \cdot 10^{11}$ | 0.410    | 0  | 23.59          |
| 014 | $3.43 \cdot 10^9$    | $3.35 \cdot 10^8$ | $2.91 \cdot 10^9$ | $8.65 \cdot 10^7$ | $2.88 \cdot 10^7$ | $1.07 \cdot 10^7$ | 1.000        | $3.43 \cdot 10^9$    | 0.602    | 0  | 8.83           |
| 015 | $1.03 \cdot 10^{10}$ | $1.98 \cdot 10^8$ | $1.05 \cdot 10^9$ | $2.33 \cdot 10^8$ | $1.66 \cdot 10^8$ | $4.98 \cdot 10^7$ | 0.504        | $5.17 \cdot 10^9$    | 0.535    | 0  | 17.98          |
| 016 | $3.03 \cdot 10^{10}$ | $3.64 \cdot 10^8$ | $1.70 \cdot 10^8$ | $7.78 \cdot 10^7$ | $8.91 \cdot 10^7$ | $2.12 \cdot 10^8$ | 0.758        | $2.30 \cdot 10^{10}$ | 0.461    | 1  | 18.20          |
| 017 | $1.00 \cdot 10^{11}$ | $4.38 \cdot 10^8$ | 0                 | 0                 | 0                 | 0                 | 0.047        | $4.68 \cdot 10^9$    | 0.298    | 1  | 10.43          |
| 018 | $2.64 \cdot 10^9$    | $3.11 \cdot 10^8$ | $1.62 \cdot 10^9$ | $2.12 \cdot 10^8$ | $1.50 \cdot 10^7$ | $1.27 \cdot 10^7$ | 0.183        | $4.83 \cdot 10^8$    | 0.821    | 0  | 5.00           |
| 019 | $6.38 \cdot 10^8$    | $3.40 \cdot 10^8$ | $1.60 \cdot 10^8$ | $7.65 \cdot 10^7$ | $3.72 \cdot 10^6$ | $1.55 \cdot 10^5$ | 0.463        | $2.96 \cdot 10^8$    | 0.859    | 1  | 9.15           |
| 020 | $1.00 \cdot 10^{11}$ | $3.45 \cdot 10^8$ | $5.19 \cdot 10^8$ | $5.34 \cdot 10^8$ | $2.20 \cdot 10^8$ | $1.06 \cdot 10^8$ | 1.000        | $1.00 \cdot 10^{11}$ | 0.712    | 1  | 24.54          |
| 021 | $1.47 \cdot 10^{11}$ | $2.96 \cdot 10^8$ | 0                 | $6.55 \cdot 10^5$ | $1.40 \cdot 10^6$ | $2.25 \cdot 10^6$ | 0.004        | $6.41 \cdot 10^8$    | 0.366    | 1  | 5.57           |
| 022 | $3.53 \cdot 10^{10}$ | $2.03 \cdot 10^8$ | $7.23 \cdot 10^7$ | $6.51 \cdot 10^5$ | $1.06 \cdot 10^6$ | $3.50 \cdot 10^5$ | 0.196        | $6.94 \cdot 10^9$    | 0.487    | 1  | 21.26          |
| 023 | $3.55 \cdot 10^8$    | $2.09 \cdot 10^8$ | $8.84 \cdot 10^8$ | $2.82 \cdot 10^8$ | $1.20 \cdot 10^8$ | $1.32 \cdot 10^8$ | 0.701        | $2.49 \cdot 10^8$    | 0.803    | 0  | 2.99           |
| 024 | $3.81 \cdot 10^{10}$ | $2.90 \cdot 10^8$ | $9.43 \cdot 10^6$ | $3.74 \cdot 10^7$ | $1.95 \cdot 10^6$ | 0                 | 0.519        | $1.98 \cdot 10^{10}$ | 0.472    | 1  | 18.20          |
| 025 | $1.09 \cdot 10^{11}$ | $3.40 \cdot 10^8$ | $1.11 \cdot 10^8$ | $2.45 \cdot 10^9$ | $2.93 \cdot 10^9$ | $3.13 \cdot 10^9$ | 0.998        | $1.09 \cdot 10^{11}$ | 0.693    | 1  | 25.74          |
| 026 | $5.18 \cdot 10^{10}$ | $3.50 \cdot 10^8$ | $1.03 \cdot 10^7$ | $1.18 \cdot 10^8$ | $6.18 \cdot 10^7$ | $3.22 \cdot 10^7$ | 0.016        | $8.27 \cdot 10^8$    | 0.358    | 0  | 3.96           |
| 027 | $2.27 \cdot 10^{10}$ | $3.10 \cdot 10^8$ | $1.20 \cdot 10^7$ | $1.62 \cdot 10^8$ | $6.34 \cdot 10^7$ | 0                 | 0.946        | $2.15 \cdot 10^{10}$ | 0.725    | 1  | 18.50          |

**Table S7:** Processed data summary: Tumor characteristics and CAR T-cell response. The table includes initial tumor burden ( $B_0$ ) and estimated CAR T-cell quantification at different time points (days 0, 7, 14, 21, and 28) in number of cells. Tumor sphericity properties are also reported: propMinSpher (proportion of the tumor volume with the minimum sphericity), cellMinSpher (number of tumor cells corresponding to the lowest observed sphericity), minSpher (minimum recorded sphericity value), and SUVmaxMinSpher (maximum standardized uptake value for the lesion with the lowest sphericity). Additionally, the overall progression status (PS) is provided, where 1 indicates progression and 0 indicates no progression. Missing values in the original dataset were handled using the method described in Section (4.4). Patients 28 to 60 are listed here.

| ID  | $B_0$ (cells)        | $C_0$ (cells)     | day7 (cells)      | day14 (cells)     | day21 (cells)        | day28 (cells)     | propMinSpher | cellsMinSpher        | minSpher | PS | SUVmaxMinSpher |
|-----|----------------------|-------------------|-------------------|-------------------|----------------------|-------------------|--------------|----------------------|----------|----|----------------|
| 028 | $7.85 \cdot 10^{10}$ | $4.20 \cdot 10^8$ | $1.88 \cdot 10^8$ | $4.71 \cdot 10^7$ | $2.62 \cdot 10^6$    | 0                 | 0.045        | $3.56 \cdot 10^9$    | 0.465    | 0  | 11.31          |
| 032 | $5.35 \cdot 10^{10}$ | $3.62 \cdot 10^8$ | $1.53 \cdot 10^8$ | $1.91 \cdot 10^9$ | $1.22 \cdot 10^{10}$ | $5.16 \cdot 10^9$ | 0.581        | $3.11 \cdot 10^{10}$ | 0.458    | 1  | 18.63          |
| 033 | $2.48 \cdot 10^{11}$ | $3.30 \cdot 10^8$ | $1.15 \cdot 10^8$ | $3.32 \cdot 10^9$ | $6.85 \cdot 10^8$    | $1.73 \cdot 10^9$ | 0.818        | $2.03 \cdot 10^{11}$ | 0.162    | 1  | 19.19          |
| 034 | $9.98 \cdot 10^9$    | $2.58 \cdot 10^8$ | $9.74 \cdot 10^9$ | $6.48 \cdot 10^8$ | $3.00 \cdot 10^8$    | $2.37 \cdot 10^8$ | 0.299        | $2.98 \cdot 10^9$    | 0.647    | 1  | 15.35          |
| 037 | $1.14 \cdot 10^9$    | $3.70 \cdot 10^8$ | $5.45 \cdot 10^8$ | $7.00 \cdot 10^5$ | $7.05 \cdot 10^5$    | $9.63 \cdot 10^5$ | 1.000        | $1.14 \cdot 10^9$    | 0.858    | 1  | 10.64          |
| 038 | $2.37 \cdot 10^{10}$ | $3.73 \cdot 10^8$ | $6.45 \cdot 10^7$ | $6.61 \cdot 10^6$ | $1.70 \cdot 10^6$    | $3.70 \cdot 10^6$ | 1.000        | $2.37 \cdot 10^{10}$ | 0.722    | 1  | 31.16          |
| 039 | $3.60 \cdot 10^9$    | $2.90 \cdot 10^8$ | $1.70 \cdot 10^8$ | $3.22 \cdot 10^8$ | $3.12 \cdot 10^8$    | $2.64 \cdot 10^8$ | 1.000        | $3.60 \cdot 10^9$    | 0.708    | 0  | 6.81           |
| 040 | $4.08 \cdot 10^{11}$ | $4.10 \cdot 10^8$ | $1.95 \cdot 10^8$ | $2.46 \cdot 10^8$ | $4.25 \cdot 10^8$    | $3.10 \cdot 10^9$ | 0.852        | $3.48 \cdot 10^{11}$ | 0.449    | 1  | 49.31          |
| 042 | $1.84 \cdot 10^{11}$ | $5.00 \cdot 10^8$ | 0                 | $7.67 \cdot 10^7$ | $9.22 \cdot 10^6$    | $1.19 \cdot 10^6$ | 0.436        | $8.04 \cdot 10^{10}$ | 0.470    | 1  | 19.57          |
| 045 | $4.73 \cdot 10^{10}$ | $2.00 \cdot 10^8$ | $6.02 \cdot 10^6$ | $2.35 \cdot 10^7$ | $1.45 \cdot 10^6$    | $8.41 \cdot 10^5$ | 1.000        | $4.73 \cdot 10^{10}$ | 0.406    | 1  | 19.62          |
| 048 | $6.04 \cdot 10^{11}$ | $2.33 \cdot 10^8$ | $1.13 \cdot 10^8$ | $3.61 \cdot 10^7$ | $1.81 \cdot 10^7$    | $4.87 \cdot 10^7$ | 0.995        | $6.02 \cdot 10^{11}$ | 0.488    | 1  | 15.13          |
| 049 | $3.00 \cdot 10^9$    | $3.35 \cdot 10^8$ | $3.54 \cdot 10^8$ | $9.01 \cdot 10^7$ | $5.78 \cdot 10^7$    | $2.98 \cdot 10^7$ | 0.685        | $2.06 \cdot 10^9$    | 0.387    | 0  | 4.17           |
| 050 | $6.61 \cdot 10^9$    | $2.90 \cdot 10^8$ | 0                 | $6.67 \cdot 10^6$ | $9.43 \cdot 10^5$    | $2.34 \cdot 10^5$ | 0.623        | $4.12 \cdot 10^9$    | 0.198    | 1  | 4.62           |
| 051 | $4.14 \cdot 10^{10}$ | $3.20 \cdot 10^8$ | $6.83 \cdot 10^8$ | $3.36 \cdot 10^8$ | $4.63 \cdot 10^7$    | $3.29 \cdot 10^6$ | 0.964        | $3.99 \cdot 10^{10}$ | 0.410    | 0  | 21.25          |
| 053 | $6.50 \cdot 10^{10}$ | $3.53 \cdot 10^8$ | $1.26 \cdot 10^9$ | $3.26 \cdot 10^9$ | $7.47 \cdot 10^8$    | $5.54 \cdot 10^8$ | 0.097        | $6.31 \cdot 10^9$    | 0.409    | 0  | 14.54          |
| 054 | $5.10 \cdot 10^{11}$ | $3.18 \cdot 10^8$ | $2.36 \cdot 10^8$ | $1.82 \cdot 10^8$ | $3.07 \cdot 10^7$    | $1.25 \cdot 10^8$ | 0.978        | $4.98 \cdot 10^{11}$ | 0.411    | 1  | 28.67          |
| 055 | $1.19 \cdot 10^{11}$ | $3.50 \cdot 10^8$ | $4.64 \cdot 10^9$ | $4.43 \cdot 10^8$ | $3.15 \cdot 10^8$    | $1.03 \cdot 10^8$ | 0.154        | $1.83 \cdot 10^{10}$ | 0.436    | 0  | 12.49          |
| 056 | $8.75 \cdot 10^{10}$ | $3.50 \cdot 10^8$ | $1.84 \cdot 10^8$ | $2.32 \cdot 10^8$ | $1.41 \cdot 10^8$    | $8.06 \cdot 10^7$ | 0.811        | $7.09 \cdot 10^{10}$ | 0.554    | 1  | 22.36          |
| 057 | $3.29 \cdot 10^8$    | $3.70 \cdot 10^8$ | $2.57 \cdot 10^8$ | $2.94 \cdot 10^7$ | $1.31 \cdot 10^7$    | $9.24 \cdot 10^6$ | 1.000        | $3.29 \cdot 10^8$    | 0.887    | 1  | 9.45           |
| 058 | $2.18 \cdot 10^{10}$ | $3.56 \cdot 10^8$ | $3.33 \cdot 10^8$ | $1.34 \cdot 10^8$ | $4.90 \cdot 10^7$    | $1.38 \cdot 10^7$ | 0.550        | $1.20 \cdot 10^{10}$ | 0.401    | 1  | 13.20          |
| 059 | $1.09 \cdot 10^{11}$ | $3.79 \cdot 10^8$ | $1.74 \cdot 10^9$ | $5.95 \cdot 10^8$ | $9.05 \cdot 10^7$    | $2.55 \cdot 10^7$ | 0.081        | $8.85 \cdot 10^9$    | 0.465    | 1  | 29.16          |
| 060 | $2.81 \cdot 10^{11}$ | $3.76 \cdot 10^8$ | $3.30 \cdot 10^8$ | $2.59 \cdot 10^8$ | $4.32 \cdot 10^7$    | $2.67 \cdot 10^7$ | 0.818        | $2.30 \cdot 10^{11}$ | 0.394    | 0  | 20.40          |

**Table S8:** Processed data summary: Tumor characteristics and CAR T-cell response. The table includes initial tumor burden ( $B_0$ ) and estimated CAR T-cell quantification at different time points (days 0, 7, 14, 21, and 28) in number of cells. Tumor sphericity properties are also reported: propMinSpher (proportion of the tumor volume with the minimum sphericity), cellMinSpher (number of tumor cells corresponding to the lowest observed sphericity), minSpher (minimum recorded sphericity value), and SUVmaxMinSpher (maximum standardized uptake value for the lesion with the lowest sphericity). Additionally, the overall progression status (PS) is provided, where 1 indicates progression and 0 indicates no progression. Missing values in the original dataset were handled using the method described in Section (4.4). Patients 61 to 79 are listed here.

| ID  | $B_0$ (cells)        | $C_0$ (cells)     | day7 (cells)      | day14 (cells)     | day21 (cells)     | day28 (cells)     | propMinSpher | cell                 | minSpher | PS | SUVmaxMinSpher |
|-----|----------------------|-------------------|-------------------|-------------------|-------------------|-------------------|--------------|----------------------|----------|----|----------------|
| 061 | $3.70 \cdot 10^9$    | $3.14 \cdot 10^8$ | $8.09 \cdot 10^9$ | $9.23 \cdot 10^8$ | $5.37 \cdot 10^8$ | $2.21 \cdot 10^8$ | 0.089        | $3.30 \cdot 10^8$    | 0.399    | 0  | 3.21           |
| 062 | $1.57 \cdot 10^8$    | $3.12 \cdot 10^8$ | $4.66 \cdot 10^8$ | $6.24 \cdot 10^8$ | $2.45 \cdot 10^8$ | $1.09 \cdot 10^8$ | 1.000        | $1.57 \cdot 10^8$    | 0.811    | 0  | 3.12           |
| 063 | $4.60 \cdot 10^9$    | $3.41 \cdot 10^8$ | $4.79 \cdot 10^8$ | $4.78 \cdot 10^8$ | $1.55 \cdot 10^8$ | $8.42 \cdot 10^5$ | 0.503        | $2.31 \cdot 10^9$    | 0.771    | 1  | 24.16          |
| 064 | $1.21 \cdot 10^{11}$ | $2.23 \cdot 10^8$ | $6.20 \cdot 10^7$ | $5.55 \cdot 10^9$ | $5.22 \cdot 10^8$ | $1.90 \cdot 10^8$ | 0.470        | $5.68 \cdot 10^{10}$ | 0.495    | 0  | 18.68          |
| 066 | $1.66 \cdot 10^{11}$ | $2.45 \cdot 10^8$ | $1.60 \cdot 10^8$ | $6.04 \cdot 10^7$ | $5.50 \cdot 10^7$ | $3.06 \cdot 10^7$ | 0.111        | $1.84 \cdot 10^{10}$ | 0.390    | 1  | 8.82           |
| 067 | $1.28 \cdot 10^9$    | $2.92 \cdot 10^8$ | $5.17 \cdot 10^8$ | $9.31 \cdot 10^7$ | $1.34 \cdot 10^7$ | $2.91 \cdot 10^7$ | 1.000        | $1.28 \cdot 10^9$    | 0.754    | 1  | 11.63          |
| 068 | $1.62 \cdot 10^{11}$ | $3.37 \cdot 10^8$ | $3.48 \cdot 10^9$ | $2.28 \cdot 10^8$ | $4.16 \cdot 10^7$ | $1.09 \cdot 10^8$ | 0.813        | $1.32 \cdot 10^{11}$ | 0.375    | 1  | 11.24          |
| 069 | $7.62 \cdot 10^7$    | $3.17 \cdot 10^8$ | $1.32 \cdot 10^8$ | $5.75 \cdot 10^7$ | $6.33 \cdot 10^7$ | $5.04 \cdot 10^7$ | 1.000        | $7.62 \cdot 10^7$    | 0.874    | 0  | 3.35           |
| 070 | $6.55 \cdot 10^9$    | $2.77 \cdot 10^8$ | $4.48 \cdot 10^8$ | $4.57 \cdot 10^6$ | $5.76 \cdot 10^5$ | $6.93 \cdot 10^5$ | 1.000        | $6.55 \cdot 10^9$    | 0.875    | 1  | 27.52          |
| 071 | $6.85 \cdot 10^9$    | $2.64 \cdot 10^8$ | $2.21 \cdot 10^8$ | $9.45 \cdot 10^7$ | $8.55 \cdot 10^6$ | $5.88 \cdot 10^6$ | 0.964        | $6.60 \cdot 10^9$    | 0.805    | 0  | 13.33          |
| 072 | $2.45 \cdot 10^9$    | $2.63 \cdot 10^8$ | $5.05 \cdot 10^9$ | $1.01 \cdot 10^9$ | $2.37 \cdot 10^8$ | $3.42 \cdot 10^8$ | 1.000        | $2.45 \cdot 10^9$    | 0.674    | 0  | 5.95           |
| 073 | $1.02 \cdot 10^{11}$ | $3.01 \cdot 10^8$ | $1.66 \cdot 10^8$ | $3.35 \cdot 10^7$ | $2.75 \cdot 10^7$ | $8.28 \cdot 10^6$ | 1.000        | $1.02 \cdot 10^{11}$ | 0.549    | 0  | 20.70          |
| 074 | $1.36 \cdot 10^{11}$ | $3.31 \cdot 10^8$ | $3.53 \cdot 10^8$ | $3.19 \cdot 10^8$ | $1.12 \cdot 10^8$ | $2.88 \cdot 10^7$ | 0.946        | $1.29 \cdot 10^{11}$ | 0.371    | 0  | 12.78          |
| 076 | $5.28 \cdot 10^9$    | $3.03 \cdot 10^8$ | $3.88 \cdot 10^8$ | $4.71 \cdot 10^8$ | $3.89 \cdot 10^8$ | $1.88 \cdot 10^8$ | 0.666        | $3.52 \cdot 10^9$    | 0.645    | 1  | 12.52          |
| 077 | $1.62 \cdot 10^9$    | $3.83 \cdot 10^8$ | $1.56 \cdot 10^8$ | $9.65 \cdot 10^7$ | $3.05 \cdot 10^7$ | $3.85 \cdot 10^6$ | 0.370        | $6.02 \cdot 10^8$    | 0.331    | 0  | 3.38           |
| 079 | $1.18 \cdot 10^{10}$ | $4.98 \cdot 10^8$ | $1.17 \cdot 10^9$ | $7.88 \cdot 10^8$ | $1.78 \cdot 10^8$ | $3.58 \cdot 10^7$ | 1.000        | $1.18 \cdot 10^{10}$ | 0.631    | 0  | 24.23          |

**Table S9:** Parameter estimation results for individual patients. The table presents the following estimated parameters:  $q_{ori}$  ( $\text{cells}^{-1} \text{ day}^{-1}$ ),  $j_{ori}$  ( $\text{day}^{-1}$ ),  $a$  ( $\text{day}^{-1}$ ), and  $\Psi^{-1}$ . The "res" column indicates the value of the predefined objective function for each patient. The parameter estimation method is detailed in Section (4.4). Patients 1 to 40 are listed here.

| Patient ID | $q_{ori}$ ( $\text{cells}^{-1} \text{ day}^{-1}$ ) | $j_{ori}$ ( $\text{day}^{-1}$ ) | $a$ ( $\text{day}^{-1}$ ) | $\Psi^{-1}$ | res         |
|------------|----------------------------------------------------|---------------------------------|---------------------------|-------------|-------------|
| 001        | $4.22444 \cdot 10^{-9}$                            | 0.236605923                     | 0.246318832               | 46.25380419 | 0.484785513 |
| 002        | $2.57273 \cdot 10^{-9}$                            | 0.287672479                     | 0.165631085               | 25.48525409 | 0.249105933 |
| 004        | $3.83995 \cdot 10^{-9}$                            | 0.012687665                     | 0.4757271                 | 2.732062503 | 0.261234172 |
| 005        | $2.57154 \cdot 10^{-9}$                            | 0.095195604                     | 0.250435634               | 1.00002011  | 0.05448324  |
| 006        | $4.09367 \cdot 10^{-8}$                            | 0.146691174                     | 0.134615002               | 5.068377794 | 0.000150883 |
| 007        | $8.68815 \cdot 10^{-9}$                            | 0.410762406                     | 0.355727106               | 1.067281892 | 0.22779413  |
| 008        | $5.58209 \cdot 10^{-9}$                            | 0.67728279                      | 0.088628495               | 6.828103989 | 0.340333577 |
| 009        | $6.40768 \cdot 10^{-9}$                            | 0.232362851                     | 0.250699645               | 58.20839338 | 0.017203985 |
| 010        | $1.42295 \cdot 10^{-9}$                            | 0.134813983                     | 0.339428711               | 73.60077187 | 0.654171017 |
| 011        | $8.82116 \cdot 10^{-9}$                            | 1.209305251                     | 0.151962471               | 7.545038169 | 2.324926471 |
| 012        | $1.57037 \cdot 10^{-9}$                            | 0.538950426                     | 0.5                       | 1           | 0.767235488 |
| 014        | $1.49147 \cdot 10^{-8}$                            | 0.223806433                     | 0.120990104               | 17.23717353 | 20.66501453 |
| 015        | $9.8926 \cdot 10^{-9}$                             | 0.244413355                     | 0.101854105               | 3.917651592 | 2.243233428 |
| 016        | $1.40679 \cdot 10^{-9}$                            | 0.28896467                      | 0.240139666               | 70.88350217 | 0.117729299 |
| 017        | $9.81988 \cdot 10^{-9}$                            | 0.298016279                     | 0.17942451                | 8.215370193 | 0.599190087 |
| 018        | $6.42657 \cdot 10^{-8}$                            | 0.213199571                     | 0.194851788               | 1.349359299 | 5.369854987 |
| 019        | $9.96337 \cdot 10^{-8}$                            | 0.212337927                     | 0.15378517                | 5.66749965  | 0.101685943 |
| 020        | $3.84589 \cdot 10^{-9}$                            | 0.200065289                     | 0.197355115               | 1.00016197  | 0.125757176 |
| 021        | $3.73343 \cdot 10^{-9}$                            | 0.014397762                     | 0.473902522               | 2.569556079 | 0.273896449 |
| 022        | $5.37287 \cdot 10^{-9}$                            | 0.125657088                     | 0.327872823               | 7.270523548 | 0.053407723 |
| 023        | $1.96973 \cdot 10^{-7}$                            | 0.179647067                     | 0.08983632                | 1.099960329 | 1.450224193 |
| 024        | $7.58159 \cdot 10^{-10}$                           | 0.198070073                     | 0.275228259               | 107.8391852 | 0.246061031 |
| 025        | $2.07834 \cdot 10^{-9}$                            | 0.73552605                      | 0.296810219               | 6.06681395  | 0.45066604  |
| 026        | $5.18392 \cdot 10^{-10}$                           | 0.036202823                     | 0.118985007               | 39.13391743 | 0.361233913 |
| 027        | $1.31935 \cdot 10^{-9}$                            | 0.155868462                     | 0.162819659               | 121.0700509 | 0.317507078 |
| 028        | $5.28727 \cdot 10^{-9}$                            | 0.554513911                     | 0.14617157                | 6.995913093 | 0.167563943 |
| 032        | $2.25801 \cdot 10^{-9}$                            | 0.409978593                     | 0.334531857               | 1.000000041 | 10.09448058 |
| 033        | $1.85268 \cdot 10^{-9}$                            | 0.568503313                     | 0.5                       | 1.000000119 | 8.709952891 |
| 034        | $2.34743 \cdot 10^{-8}$                            | 0.319207569                     | 0.11245112                | 1.624580094 | 281.3514812 |
| 037        | $3.5484 \cdot 10^{-8}$                             | 0.133699484                     | 0.147460474               | 425.5154941 | 0.095483342 |
| 038        | $1.71524 \cdot 10^{-9}$                            | 0.23237352                      | 0.248061933               | 339.6916321 | 0.297434311 |
| 039        | $1.30803 \cdot 10^{-8}$                            | 0.260953398                     | 0.176074106               | 7.456575215 | 0.045046642 |
| 040        | $3.99085 \cdot 10^{-10}$                           | 0.271462195                     | 0.028205017               | 13.5063091  | 0.637929981 |

**Table S10:** Parameter estimation results for individual patients. The table presents the following estimated parameters:  $q_{ori}$  ( $\text{cells}^{-1} \text{ day}^{-1}$ ),  $j_{ori}$  ( $\text{day}^{-1}$ ),  $a$  ( $\text{day}^{-1}$ ), and  $\Psi^{-1}$ . The "res" column indicates the value of the predefined objective function for each patient. The parameter estimation method is detailed in Section (4.4). Patients 42 to 79 are listed here.

| Patient ID | $q_{ori}$ ( $\text{cells}^{-1} \text{ day}^{-1}$ ) | $j_{ori}$ ( $\text{day}^{-1}$ ) | $a$ ( $\text{day}^{-1}$ ) | $\Psi^{-1}$ | res         |
|------------|----------------------------------------------------|---------------------------------|---------------------------|-------------|-------------|
| 042        | $3.10841 \cdot 10^{-9}$                            | 0.092111701                     | 0.362464922               | 1.448859683 | 0.78173083  |
| 045        | $7.34265 \cdot 10^{-9}$                            | 0.604303418                     | 0.09496014                | 8.046990222 | 0.117632204 |
| 048        | $2.96236 \cdot 10^{-9}$                            | 0.230560947                     | 0.252081743               | 1.320539699 | 0.053476698 |
| 049        | $1.3706 \cdot 10^{-8}$                             | 0.230631704                     | 0.178738319               | 23.37990871 | 0.001114808 |
| 050        | $4.57985 \cdot 10^{-9}$                            | 0.190943099                     | 0.282269953               | 215.0359242 | 0.262884879 |
| 051        | $1.54042 \cdot 10^{-9}$                            | 0.243193352                     | 0.236022111               | 8.632542956 | 0.412150712 |
| 053        | $5.61624 \cdot 10^{-9}$                            | 0.794063722                     | 0.303546705               | 2.898667695 | 3.511993658 |
| 054        | $1.45624 \cdot 10^{-10}$                           | 0.104381686                     | 0.010092295               | 26.11443426 | 0.045274184 |
| 055        | $7.77444 \cdot 10^{-10}$                           | 0.1367629                       | 0.150311409               | 3.947596521 | 57.58718702 |
| 056        | $4.19851 \cdot 10^{-9}$                            | 0.147931215                     | 0.023432991               | 2.385601315 | 0.085870032 |
| 057        | $1.26442 \cdot 10^{-7}$                            | 0.088960621                     | 0.066534822               | 19.64603961 | 0.039866894 |
| 058        | $1.01306 \cdot 10^{-8}$                            | 0.232236567                     | 0.030713766               | 4.801097565 | 0.001599882 |
| 059        | $2.98991 \cdot 10^{-9}$                            | 0.245919188                     | 0.26013751                | 1.375983674 | 5.80994767  |
| 060        | $1.75542 \cdot 10^{-9}$                            | 0.113843232                     | 0.19877519                | 1.346393528 | 0.008614917 |
| 061        | $1.21662 \cdot 10^{-7}$                            | 0.58927079                      | 0.142457958               | 1.056680405 | 189.3592369 |
| 062        | $3.84414 \cdot 10^{-11}$                           | 0.053563187                     | 0.033045243               | 9.615610683 | 0.468101475 |
| 063        | $1.60274 \cdot 10^{-8}$                            | 0.313230806                     | 0.223306803               | 4.324381655 | 0.059263037 |
| 064        | $3.85798 \cdot 10^{-9}$                            | 0.787828809                     | 0.399476981               | 1.310549209 | 0.194277426 |
| 066        | $1.24274 \cdot 10^{-10}$                           | 0.010030689                     | 0.040449422               | 99.39123075 | 0.023069125 |
| 067        | $9.62776 \cdot 10^{-8}$                            | 0.011262764                     | 0.013166118               | 1.579000855 | 0.159113107 |
| 068        | $2.24764 \cdot 10^{-9}$                            | 0.01125592                      | 0.01963634                | 1.184095455 | 30.93634051 |
| 069        | $2.41756 \cdot 10^{-7}$                            | 0.010295727                     | 0.430335859               | 19.4457565  | 0.106886595 |
| 070        | $4.42419 \cdot 10^{-9}$                            | 0.192742419                     | 0.286835752               | 183.4949035 | 0.091347746 |
| 071        | $5.05083 \cdot 10^{-9}$                            | 0.255510915                     | 0.227766194               | 24.6857117  | 0.00585953  |
| 072        | $1.73545 \cdot 10^{-7}$                            | 0.744099104                     | 0.185953995               | 1.09736522  | 72.05982314 |
| 073        | $3.16073 \cdot 10^{-9}$                            | 0.027836482                     | 0.435503936               | 1.593820364 | 0.059695974 |
| 074        | $2.21784 \cdot 10^{-9}$                            | 0.120366858                     | 0.176344378               | 1.358832037 | 0.00297919  |
| 076        | $4.25153 \cdot 10^{-8}$                            | 0.302784782                     | 0.095514845               | 1.522944265 | 0.025437198 |
| 077        | $3.74577 \cdot 10^{-8}$                            | 0.189767873                     | 0.102597304               | 9.815625234 | 0.1618505   |
| 079        | $1.30712 \cdot 10^{-8}$                            | 0.312157338                     | 0.222237032               | 2.35396856  | 1.41558107  |

**Table S11:** Quantitative PET imaging parameters for individual patients, including maximum standardized uptake value (maxSUVmax), metabolic tumor volume (totalMTV), and total lesion glycolysis (tTLG). Spherical shape descriptors include maxSpher (the highest sphericity observed in lesions), volMaxSpher (the volume of the lesion with maxSpher), SUVmaxMaxSpher (the maximum SUV within volMaxSpher), minSpher (the lowest sphericity observed in lesions), volMinSpher (the volume of the lesion with minSpher), and SUVmaxMinSpher (the maximum SUV within volMinSpher). A multivariate model, incorporating these covariates, was employed for statistical analysis in Section 3. Data for patients 1 to 27 are presented.

| ID  | SUVmax      | tMTV    | tTLG        | maxSpher  | volMaxSpher | SUVmaxMaxSpher | minSpher  | volMinSpher | SUVmaxMinSpher |
|-----|-------------|---------|-------------|-----------|-------------|----------------|-----------|-------------|----------------|
| 001 | 31.14040958 | 46428   | 497997.8617 | 0.670873  | 46428       | 31.14040958    | 0.670873  | 46428       | 31.14040958    |
| 002 | 30.31829686 | 70667   | 456245.8835 | 0.915839  | 4431        | 25.55203391    | 0.6582204 | 25554       | 30.31829686    |
| 004 | 18.19751294 | 611544  | 5246529.587 | 0.9026096 | 7145        | 9.389399772    | 0.4953979 | 86539       | 14.13145418    |
| 005 | 29.33585022 | 463468  | 6184989.29  | 0.8416696 | 1704        | 10.8892163     | 0.5371611 | 305708      | 29.33585022    |
| 006 | 8.403944516 | 6438    | 21404.02074 | 0.7720055 | 2490        | 7.655044036    | 0.6019998 | 3562        | 8.403944516    |
| 007 | 13.41014431 | 73449   | 440552.4533 | 0.6668241 | 23028       | 11.197646      | 0.5675628 | 3322        | 5.345828601    |
| 008 | 34.61982966 | 325919  | 2384376.599 | 0.9158157 | 1360        | 4.928512336    | 0.3943484 | 6104        | 7.589016914    |
| 009 | 4.196204828 | 29338   | 65537.70387 | 0.854696  | 20899       | 4.196204828    | 0.816125  | 8439        | 4.07632141     |
| 010 | 23.88173769 | 123637  | 731397.5558 | 0.8910394 | 1157        | 8.302023429    | 0.5095685 | 68369       | 23.88173769    |
| 011 | 37.00585999 | 228031  | 1777634.479 | 0.9161876 | 1383        | 12.0447112     | 0.3276484 | 3739        | 8.905750773    |
| 012 | 23.58769118 | 1681641 | 11423774.55 | 0.9014572 | 1337        | 17.40650213    | 0.4097244 | 581491      | 23.58769118    |
| 014 | 8.827870018 | 14371   | 48612.08542 | 0.6024752 | 14371       | 8.827870018    | 0.6024752 | 14371       | 8.827870018    |
| 015 | 17.98455261 | 43023   | 276634.0592 | 0.8454768 | 1582        | 9.847171389    | 0.5348043 | 21676       | 17.98455261    |
| 016 | 18.20275268 | 127122  | 784637.9868 | 0.8195118 | 2144        | 9.25605181     | 0.4612064 | 96320       | 18.20275268    |
| 017 | 89.27109066 | 420454  | 9596417.211 | 0.8915491 | 3320        | 14.30505057    | 0.2978963 | 19586       | 10.42684123    |
| 018 | 6.68801613  | 11040   | 48447.80035 | 0.838826  | 9016        | 6.68801613     | 0.8213215 | 2024        | 4.999610003    |
| 019 | 9.25485389  | 2673    | 13889.27552 | 0.8893692 | 1435        | 9.25485389     | 0.8586152 | 1238        | 9.145860284    |
| 020 | 24.54231507 | 419883  | 5852262.821 | 0.7120827 | 419883      | 24.54231507    | 0.7120827 | 419883      | 24.54231507    |
| 021 | 19.0886     | 615181  | 3574371.88  | 0.8823    | 4842        | 16.7362        | 0.3658    | 2687        | 5.5741         |
| 022 | 21.2628     | 147926  | 1055059.52  | 0.9327    | 282         | 2.0017         | 0.4865    | 29054       | 21.2628        |
| 023 | 2.9940      | 1487    | 3096.82     | 0.8318    | 444         | 2.0826         | 0.8031    | 1043        | 2.9940         |
| 024 | 21.4876     | 159476  | 875095.23   | 0.9144    | 1700        | 12.9502        | 0.4722    | 82847       | 18.2030        |
| 025 | 25.7368     | 456952  | 3714369.20  | 0.8946    | 1008        | 12.9945        | 0.6925    | 455944      | 25.7368        |
| 026 | 12.5787     | 216948  | 1787177.07  | 0.8842    | 981         | 3.3703         | 0.3576    | 3465        | 3.9627         |
| 027 | 18.5036     | 95196   | 625899.74   | 0.8840    | 3645        | 16.1348        | 0.7253    | 90037       | 18.5036        |

**Table S12:** Quantitative PET imaging parameters for individual patients, including maximum standardized uptake value (maxSUVmax), metabolic tumor volume (totalMTV), and total lesion glycolysis (tTLG). Spherical shape descriptors include maxSpher (the highest sphericity observed in lesions), volMaxSpher (the volume of the lesion with maxSpher), SUVmaxMaxSpher (the maximum SUV within volMaxSpher), minSpher (the lowest sphericity observed in lesions), volMinSpher (the volume of the lesion with minSpher), and SUVmaxMinSpher (the maximum SUV within volMinSpher). A multivariate model, incorporating these covariates, was employed for statistical analysis in Section 3. Data for patients 28 to 64 are presented.

| ID  | SUVmax | tMTV    | tTLG        | maxSpher | volMaxSpher | SUVmaxMaxSpher | minSpher | volMinSpher | SUVmaxMinSpher |
|-----|--------|---------|-------------|----------|-------------|----------------|----------|-------------|----------------|
| 028 | 39.79  | 328865  | 2332321.67  | 0.8863   | 22665       | 12.28          | 0.4647   | 14892       | 11.31          |
| 032 | 18.63  | 223936  | 1266200.78  | 0.8290   | 912         | 5.67           | 0.4584   | 130184      | 18.63          |
| 033 | 35.83  | 1037527 | 4095346.55  | 0.8863   | 4609        | 26.33          | 0.1617   | 848292      | 19.19          |
| 034 | 17.10  | 41813   | 197464.28   | 0.8904   | 863         | 7.57           | 0.6472   | 12482       | 15.35          |
| 037 | 10.64  | 4792    | 15826.91    | 0.8584   | 4792        | 10.64          | 0.8584   | 4792        | 10.64          |
| 038 | 31.16  | 99366   | 1029791.42  | 0.7223   | 99366       | 31.16          | 0.7223   | 99366       | 31.16          |
| 039 | 6.81   | 15066   | 47893.74    | 0.7081   | 15066       | 6.81           | 0.7081   | 15066       | 6.81           |
| 040 | 49.31  | 1708539 | 27856356.07 | 0.8344   | 152045      | 33.52          | 0.4492   | 1456170     | 49.31          |
| 042 | 24.05  | 772822  | 6348133.66  | 0.8869   | 448         | 5.14           | 0.4701   | 336889      | 19.57          |
| 045 | 19.62  | 198025  | 1202919.46  | 0.4056   | 198025      | 19.62          | 0.4056   | 198025      | 19.62          |
| 048 | 15.13  | 2531970 | 18172035.90 | 0.9054   | 3850        | 12.05          | 0.4879   | 2520275     | 15.13          |
| 049 | 10.42  | 12567   | 36722.47    | 0.8799   | 535         | 2.22           | 0.3870   | 8609        | 4.17           |
| 050 | 5.90   | 27689   | 28375.41    | 0.8554   | 1541        | 5.75           | 0.1982   | 17238       | 4.62           |
| 051 | 21.25  | 173465  | 804892.06   | 0.8560   | 1808        | 8.17           | 0.4098   | 167292      | 21.25          |
| 053 | 18.60  | 272415  | 1339984.36  | 0.8836   | 1279        | 7.57           | 0.4092   | 26445       | 14.54          |
| 054 | 28.67  | 2134739 | 18367735.31 | 0.8955   | 2183        | 15.57          | 0.4114   | 2087669     | 28.67          |
| 055 | 29.82  | 498382  | 3125080.23  | 0.8862   | 1393        | 2.00           | 0.4360   | 76556       | 12.49          |
| 056 | 22.36  | 366388  | 2823770.45  | 0.8698   | 1447        | 13.04          | 0.5540   | 297056      | 22.36          |
| 057 | 9.45   | 1377    | 5557.48     | 0.8865   | 1377        | 9.45           | 0.8865   | 1377        | 9.45           |
| 058 | 13.20  | 91462   | 459344.47   | 0.8786   | 1012        | 5.75           | 0.4014   | 50345       | 13.20          |
| 059 | 29.16  | 455636  | 3476727.89  | 0.5145   | 418574      | 19.68          | 0.4654   | 37062       | 29.16          |
| 060 | 20.40  | 1177058 | 7013039.23  | 0.9205   | 1333        | 5.25           | 0.3940   | 962397      | 20.40          |
| 061 | 16.01  | 15513   | 61597.06    | 0.8941   | 3921        | 16.01          | 0.3987   | 1381        | 3.21           |
| 062 | 3.12   | 659     | 1296.73     | 0.8115   | 659         | 3.12           | 0.8115   | 659         | 3.12           |
| 063 | 24.16  | 19262   | 119212.64   | 0.8943   | 330         | 3.25           | 0.7710   | 9689        | 24.16          |
| 064 | 25.78  | 506497  | 4353287.38  | 0.9100   | 1563        | 20.13          | 0.4954   | 237802      | 18.68          |

**Table S13:** Quantitative PET imaging parameters for individual patients, including maximum standardized uptake value (maxSUVmax), metabolic tumor volume (totalMTV), and total lesion glycolysis (tTLG). Spherical shape descriptors include maxSpher (the highest sphericity observed in lesions), volMaxSpher (the volume of the lesion with maxSpher), SUVmaxMaxSpher (the maximum SUV within volMaxSpher), minSpher (the lowest sphericity observed in lesions), volMinSpher (the volume of the lesion with minSpher), and SUVmaxMinSpher (the maximum SUV within volMinSpher). A multivariate model, incorporating these covariates, was employed for statistical analysis in Section 3. Data for patients 66 to 79 are presented.

| ID  | SUVmax  | tMTV   | tTLG        | maxSpher | volMaxSpher | SUVmaxMaxSpher | minSpher | volMinSpher | SUVmaxMinSpher |
|-----|---------|--------|-------------|----------|-------------|----------------|----------|-------------|----------------|
| 066 | 16.5972 | 696845 | 3223506.054 | 0.8580   | 1010        | 5.8231         | 0.3896   | 77080       | 8.8230         |
| 067 | 11.6276 | 5375   | 27469.5418  | 0.7542   | 5375        | 11.6276        | 0.7542   | 5375        | 11.6276        |
| 068 | 11.2449 | 678228 | 3808748.614 | 0.8707   | 2841        | 8.7785         | 0.3754   | 551719      | 11.2449        |
| 069 | 3.3476  | 319    | 824.4640    | 0.8743   | 319         | 3.3476         | 0.8743   | 319         | 3.3476         |
| 070 | 27.5193 | 27426  | 282570.5594 | 0.8754   | 27426       | 27.5193        | 0.8754   | 27426       | 27.5193        |
| 071 | 13.3260 | 28679  | 38789.7788  | 0.8625   | 1043        | 0.5467         | 0.8048   | 27636       | 13.3260        |
| 072 | 5.9520  | 10274  | 14846.7289  | 0.6740   | 10274       | 5.9520         | 0.6740   | 10274       | 5.9520         |
| 073 | 20.7003 | 428028 | 3707995.272 | 0.5492   | 428028      | 20.7003        | 0.5492   | 428028      | 20.7003        |
| 074 | 19.5549 | 569330 | 3636333.535 | 0.9057   | 591         | 3.9125         | 0.3714   | 538835      | 12.7783        |
| 076 | 12.5225 | 22127  | 113720.3108 | 0.8631   | 1230        | 7.6770         | 0.6453   | 14728       | 12.5225        |
| 077 | 12.1084 | 6805   | 22812.5687  | 0.6951   | 4284        | 12.1084        | 0.3306   | 2521        | 3.3823         |
| 079 | 24.2292 | 49625  | 395750.6399 | 0.6313   | 49625       | 24.2292        | 0.6313   | 49625       | 24.2292        |

## Supplemental References

- [1] Chen, Y.: Dynamics of Tumor-Immune Systems (2023)
